# Supplementary material for: FADE: Few-shot/zero-shot Anomaly Detection Engine using Large Vision-Language Model
Source: arXiv:2409.00556 ancillary file (2024-08-31)
Supplement: Supplementary file 1 [file supplementary.pdf]

# FADE: Few-shot/zero-shot Anomaly Detection Engine using Large Vision-Language Model

## Supplementary Material

Yuanwei Li<sup>1,2</sup>

yuanwei\_li@hotmail.com

Elizaveta Ivanova<sup>1</sup>

lisa.ivanova@entrust.com

Martins Bruveris

martins.bruveris@entrust.com

Onfido

London, UK

---

## 1 ChatGPT Prompt Ensemble

Figure 1-5 show the 5 different instruction prompts that are passed to ChatGPT 3.5 and its corresponding responses for the normal and anomalous text prompts. We vary the wording of the instructions to obtain diverse output. All the responses from the 5 instructions are combined to form the ChatGPT prompt ensemble which consists of 486 anomaly and 423 normal prompts.

---

<sup>1</sup>These authors contributed equally.

<sup>2</sup>Corresponding author.

## Instruction #1

Give 100 prompts that describe a photo of an undamaged/a defective object or texture in industrial manufacturing. Do not mention specific object name. Be diverse in adjectives and sentence structure. Give your outputs in JSON format as a list.

## Normal Response

A smooth, pristine surface gleaming under bright lights.  
 A flawless, polished texture reflecting its surroundings.  
 An immaculate, unblemished object with perfect symmetry.  
 A sleek, refined surface devoid of any imperfections.  
 A pristine, untouched material showcasing its pristine condition.  
 A seamless, faultless texture with uniform consistency.  
 A perfectly formed, unmarred object showcasing precision craftsmanship.  
 A perfectly formed, unmarred texture showcasing manufacturing expertise.  
 A flawless, impeccable texture demonstrating exceptional manufacturing standards.  
 A clean, pristine object exhibiting meticulous attention to detail.  
 A shiny, lustrous surface radiating with perfection.  
 A perfectly smooth, flawless texture devoid of any defects.  
 An unblemished, flawless object presenting excellence in manufacturing.  
 A finely crafted, flawless surface displaying superior quality.  
 A faultless, seamless texture exhibiting flawless execution.  
 A pristine, untouched object showcasing manufacturing mastery.  
 A sleek, flawless surface reflecting professional craftsmanship.  
 A flawless, polished texture with a mirror-like finish.  
 An immaculate, pristine object demonstrating precision engineering.  
 A perfectly formed, unmarred texture showcasing manufacturing expertise.  
 A spotless, gleaming surface reflecting attention to detail.  
 A flawless, impeccable material exhibiting exceptional quality.  
 A clean, pristine texture showcasing manufacturing excellence.  
 A shiny, lustrous object radiating with perfection.  
 A perfectly smooth, flawless, fragile device of any blemishes.  
 An unblemished, impeccable texture presenting superior craftsmanship.  
 A finely crafted, flawless object displaying top-notch quality.  
 A faultless, seamless surface showcasing expert manufacturing.  
 A pristine, untouched texture reflecting meticulous craftsmanship.  
 A sleek, flawless object demonstrating excellence in manufacturing.  
 A flawless, polished surface with an impeccable finish.  
 An immaculate, pristine texture showcasing superior design.  
 A perfectly formed, unmarred material reflecting precision engineering.  
 A spotless, gleaming object presenting perfection in production.  
 A flawless, impeccable texture with outstanding attention to detail.  
 A clean, pristine surface demonstrating exceptional craftsmanship.  
 A shiny, lustrous texture radiating with quality and excellence.  
 A perfectly smooth, flawless object showcasing top-tier manufacturing.  
 An unblemished, impeccable surface presenting flawless execution.  
 A finely crafted, flawless texture displaying meticulous attention to detail.  
 A faultless, seamless object reflecting excellence in design.  
 A pristine, untouched surface showcasing superior manufacturing standards.  
 A sleek, flawless texture exhibiting precision craftsmanship.  
 A flawless, polished object with a flawless finish.  
 An immaculate, pristine surface demonstrating exceptional quality.  
 A perfectly formed, unmarred texture showcasing flawless execution.  
 A spotless, gleaming material reflecting perfection in manufacturing.  
 A shiny, lustrous object presenting superior manufacturing standards.  
 A clean, pristine object presenting superior manufacturing standards.  
 A shiny, lustrous texture radiating with professionalism.  
 A perfectly smooth, flawless material with impeccable design.  
 An unblemished, impeccable object showcasing expert craftsmanship.  
 A finely crafted, flawless surface displaying precision engineering.  
 A faultless, seamless texture reflecting meticulous attention to detail.  
 A pristine, untouched object presenting top-tier manufacturing quality.  
 A sleek, flawless surface demonstrating exceptional craftsmanship.  
 A flawless, polished texture with outstanding quality.  
 An immaculate, pristine object showcasing flawless design.  
 A perfectly formed, unmarred surface reflecting expert craftsmanship.  
 A spotless, gleaming texture presenting perfection in production.  
 A flawless, impeccable object with superior manufacturing standards.  
 A clean, pristine texture exhibiting meticulous attention to detail.  
 A shiny, lustrous surface radiating with excellence.  
 A perfectly smooth, flawless object showcasing precision manufacturing.  
 An unblemished, impeccable texture reflecting flawless execution.  
 A finely crafted, flawless material presenting top-notch quality.  
 A faultless, seamless object demonstrating exceptional design.  
 A pristine, untouched texture showcasing superior craftsmanship.  
 A sleek, flawless object with impeccable attention to detail.  
 A flawless, polished surface presenting perfection in production.  
 An immaculate, pristine texture with flawless execution.  
 A perfectly formed, unmarred object reflecting superior craftsmanship.  
 A spotless, gleaming surface exhibiting precision engineering.  
 A flawless, impeccable texture with outstanding craftsmanship.  
 A clean, pristine material presenting flawless design.  
 A shiny, lustrous object radiating with top-tier quality.  
 A perfectly smooth, flawless surface showcasing expert manufacturing.  
 An unblemished, impeccable surface with exceptional attention to detail.  
 A finely crafted, flawless object presenting perfection in design.  
 A faultless, seamless texture reflecting meticulous craftsmanship.  
 A pristine, untouched surface demonstrating flawless execution.  
 A sleek, flawless texture showcasing exceptional manufacturing.  
 A flawless, polished object with superior attention to detail.

## Anomaly Response

A jagged, fragmented surface in a manufacturing setting.  
 An irregular, bumpy texture with visible cracks.  
 A warped, distorted object with uneven edges.  
 A rough, pitted surface marred by imperfections.  
 A corroded, deteriorating material showing signs of decay.  
 A mangled, twisted component with bent edges.  
 A splintered, fractured object with sharp edges.  
 A flawed, uneven surface showing signs of wear and tear.  
 A damaged, chipped texture exhibiting signs of stress.  
 A discolored, tarnished object displaying signs of degradation.  
 A rough, uneven texture with visible indentations.  
 A distorted, misshapen object with irregular contours.  
 A cracked, fissured surface revealing underlying flaws.  
 A weathered, worn-down texture showing signs of erosion.  
 A fractured, fragmented object with visible breakage.  
 A flawed, imperfect surface with visible irregularities.  
 A scratched, scuffed texture displaying signs of abrasion.  
 A deformed, contorted object with irregular shapes.  
 A deteriorating, decaying material exhibiting structural weaknesses.  
 A damaged, flawed surface with visible blemishes.  
 A warped, twisted texture displaying irregular patterns.  
 A corroded, rusted object showing signs of oxidation.  
 A cracked, shattered surface with sharp protrusions.  
 A worn, weathered texture showing signs of aging.  
 A broken, fragmented object with missing pieces.  
 A chipped, dented surface exhibiting signs of impact.  
 A flawed, defective texture with visible irregularities.  
 A disfigured, misaligned object with warped edges.  
 A pockmarked, uneven surface displaying indentations.  
 A corroded, deteriorated texture showing signs of rust.  
 A fractured, splintered object with jagged edges.  
 A rough, coarse surface marred by imperfections.  
 A warped, bent material displaying structural weaknesses.  
 A damaged, flawed texture with visible deformities.  
 A worn-down, weathered object exhibiting signs of fatigue.  
 A cracked, fissured texture showing underlying weaknesses.  
 A damaged, deteriorating surface with visible decay.  
 A deformed, misshapen object with irregular contours.  
 A flawed, imperfect texture with visible cracks.  
 A scratched, scuffed material displaying signs of wear.  
 A corroded, rusted surface exhibiting signs of corrosion.  
 A fractured, fragmented texture with visible breakage.  
 A damaged, flawed object with visible imperfections.  
 A warped, twisted surface displaying irregular patterns.  
 A cracked, shattered object with sharp edges.  
 A worn, weathered texture showing signs of erosion.  
 A broken, fragmented material with missing components.  
 A chipped, dented object exhibiting signs of damage.  
 A flawed, defective surface with visible irregularities.  
 A disfigured, misaligned texture with warped patterns.  
 A pockmarked, uneven object displaying indentations.  
 A corroded, deteriorated material showing signs of decay.  
 A fractured, splintered texture with jagged protrusions.  
 A rough, coarse object marred by surface imperfections.  
 A warped, bent texture displaying structural weaknesses.  
 A damaged, flawed surface with visible blemishes.  
 A worn-down, weathered material exhibiting signs of aging.  
 A cracked, fissured object revealing underlying flaws.  
 A corroded, rusted texture showing signs of oxidation.  
 A fractured, fragmented surface with visible breakage.  
 A damaged, flawed texture with visible deformities.  
 A disfigured, misaligned material with warped edges.  
 A rough, pitted object marred by imperfections.  
 A chipped, dented texture exhibiting signs of impact.  
 A flawed, imperfect surface with visible cracks.  
 A scratched, scuffed object displaying signs of abrasion.  
 A deformed, misshapen texture with irregular contours.  
 A deteriorating, decaying object exhibiting structural weaknesses.  
 A flawed, defective material with visible irregularities.  
 A fractured, splintered surface with sharp edges.  
 A rough, coarse texture marred by surface imperfections.  
 A damaged, flawed object with visible imperfections.  
 A warped, twisted material displaying irregular patterns.  
 A worn-down, weathered texture exhibiting signs of erosion.  
 A cracked, shattered material with sharp protrusions.  
 A broken, fragmented surface with missing pieces.  
 A chipped, dented object exhibiting signs of damage.  
 A flawed, defective texture with visible deformities.  
 A disfigured, misaligned surface with warped contours.  
 A pockmarked, uneven material displaying indentations.  
 A corroded, deteriorated object showing signs of decay.  
 A fractured, fragmented texture with visible breakage.  
 A damaged, flawed surface with visible blemishes.  
 A rough, pitted texture marred by imperfections.  
 A scratched, scuffed object displaying signs of wear.  
 A warped, bent material displaying structural weaknesses.  
 A corroded, rusted surface exhibiting signs of corrosion.  
 A fractured, splintered object with jagged protrusions.  
 A worn, weathered texture showing signs of aging.  
 A broken, fragmented material with missing components.  
 A chipped, dented surface exhibiting signs of impact.  
 A flawed, imperfect object with visible cracks.  
 A disfigured, misaligned texture with irregular patterns.

Figure 1: ChatGPT prompt ensemble 1

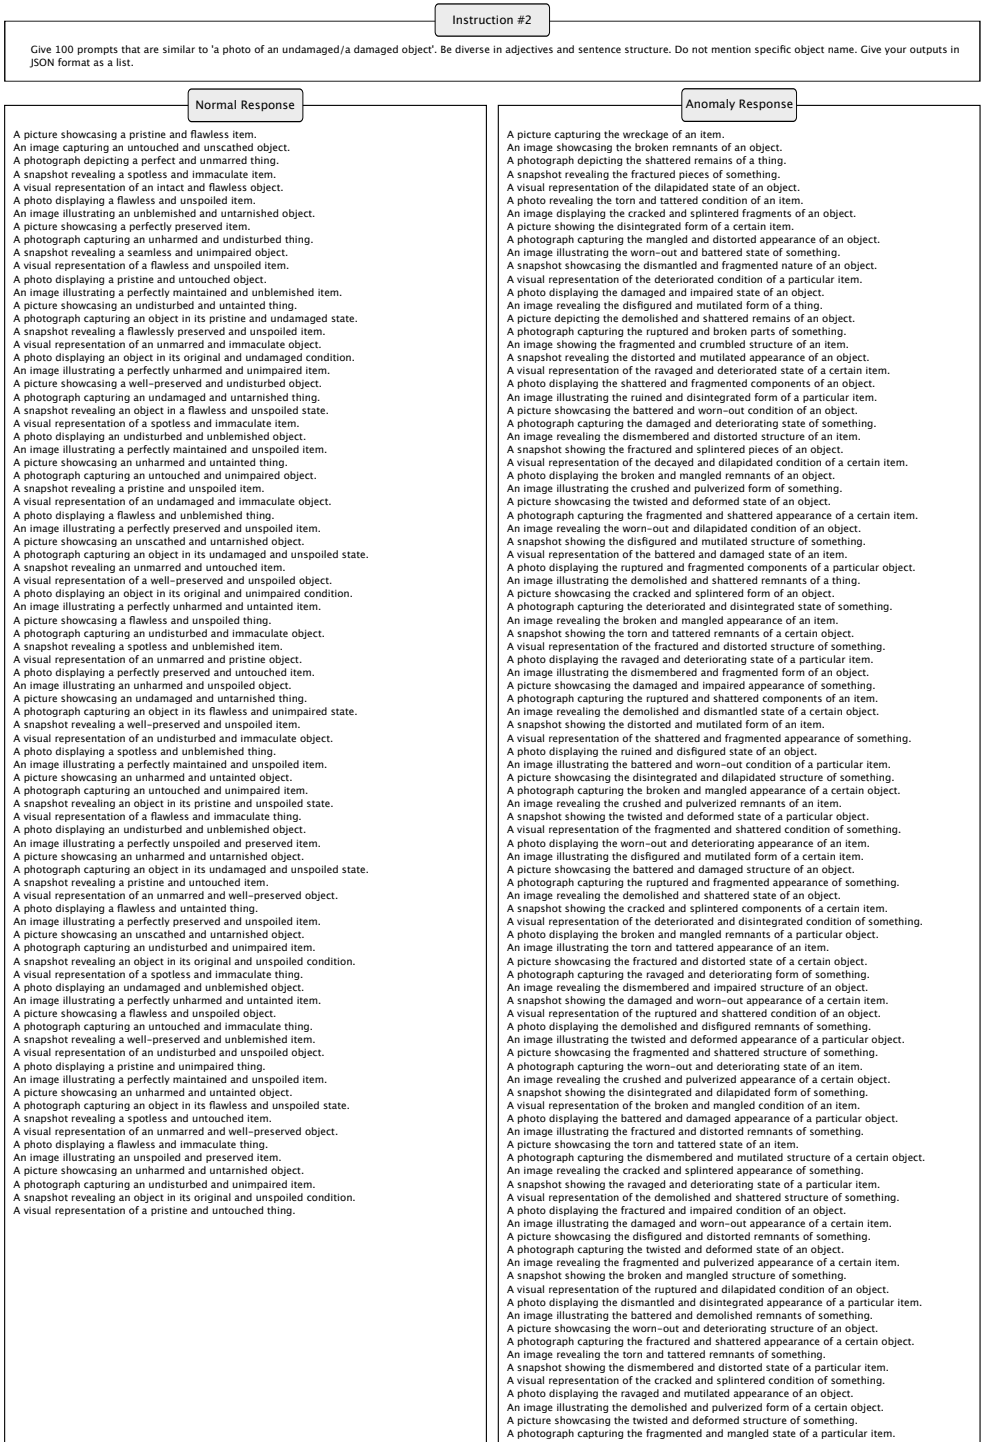

Figure 2: ChatGPT prompt ensemble 2

## Instruction #3

Give 100 prompts that describe a photo of an undamaged/a damaged object. Do not mention specific object name. Give your outputs in JSON format.

## Normal Response

A pristine object bathed in soft light.  
 An image showcasing the flawless surface of the item.  
 A photograph capturing the perfect condition of the object.  
 A picture highlighting the untouched beauty of the item.  
 An image displaying the unblemished exterior of the object.  
 A snapshot of the immaculate state of the item.  
 A photo showcasing the pristine condition of the object.  
 A close-up shot revealing the flawless craftsmanship.  
 An image displaying the object in its original, undamaged state.  
 A photograph capturing the pristine finish of the item.  
 A picture highlighting the flawless design of the object.  
 An image showcasing the untouched perfection of the item.  
 A snapshot of the object gleaming in pristine condition.  
 A photo highlighting the unmarred surface of the object.  
 A close-up shot revealing the immaculate details of the item.  
 An image displaying the object looking as good as new.  
 A photograph capturing the flawless contours of the item.  
 A picture showcasing the object without a scratch.  
 An image highlighting the perfect form of the object.  
 A snapshot of the object in its pristine glory.  
 A photo showcasing the untouched elegance of the item.  
 A close-up shot revealing the pristine finish of the object.  
 An image displaying the object in its flawless state.  
 A photograph capturing the immaculate presentation of the item.  
 A picture highlighting the undamaged surface of the object.  
 An image showcasing the object's flawless appearance.  
 A snapshot of the object showing no signs of wear.  
 A photo capturing the pristine condition of the surface.  
 A close-up shot revealing the unspooled details of the item.  
 An image displaying the object in perfect condition.  
 A photograph showcasing the flawless exterior of the item.  
 A picture highlighting the immaculate state of the object.  
 An image displaying the object looking untouched and perfect.  
 A snapshot of the object gleaming without surface damage.  
 A photo showcasing the pristine finish of the surface.  
 A close-up shot revealing the flawless contours of the item.  
 An image displaying the object without any imperfections.  
 A photograph capturing the unblemished beauty of the item.  
 A picture highlighting the untouched condition of the object.  
 An image showcasing the object's flawless presentation.  
 A snapshot of the object in its original, undamaged form.  
 A photo highlighting the immaculate craftsmanship of the item.  
 A close-up shot revealing the pristine surface of the object.  
 An image displaying the object looking as perfect as ever.  
 A photograph capturing the flawless appearance of the item.  
 A picture showcasing the object without any flaws.  
 An image highlighting the perfect state of the object.  
 A snapshot of the object in its pristine condition.  
 A photo showcasing the untouched beauty of the surface.  
 A close-up shot revealing the flawless details of the item.  
 An image displaying the object in its untouched state.  
 A photograph capturing the immaculate form of the item.  
 A picture highlighting the undamaged presentation of the object.  
 An image showcasing the object's flawless exterior.  
 A snapshot of the object looking as good as new.  
 A photo capturing the pristine condition of the item.  
 A close-up shot revealing the unmarred surface of the object.  
 An image displaying the object without any marks.  
 A photograph showcasing the untouched elegance of the item.  
 A picture highlighting the pristine finish of the object.  
 An image showcasing the object in its original, undamaged condition.  
 A snapshot of the object gleaming in perfect condition.  
 A photo showcasing the flawless surface of the item.  
 A close-up shot revealing the untouched details of the object.  
 An image displaying the object looking flawless and untouched.  
 A photograph capturing the pristine appearance of the item.  
 A picture highlighting the immaculate state of the surface.  
 An image showcasing the object without any signs of wear.  
 A snapshot of the object in its pristine state.  
 A photo highlighting the flawless craftsmanship of the item.  
 A close-up shot revealing the pristine contours of the object.  
 An image displaying the object without any imperfections.  
 A photograph showcasing the unspooled beauty of the item.  
 A picture highlighting the flawless condition of the object.  
 An image displaying the object looking as perfect as ever.  
 A snapshot of the object in its untouched state.  
 A photo showcasing the flawless presentation of the item.  
 A close-up shot revealing the perfect surface of the object.  
 An image displaying the object in its original, undamaged form.  
 A photograph capturing the flawless beauty of the item.  
 A picture highlighting the pristine appearance of the object.  
 An image showcasing the object without any flaws.  
 A snapshot of the object in its pristine glory.  
 A photo highlighting the untouched craftsmanship of the item.  
 A close-up shot revealing the unblemished surface of the object.  
 An image displaying the object looking as good as new.  
 A photograph capturing the pristine condition of the surface.  
 A picture showcasing the flawless finish of the object.  
 An image highlighting the unmarred presentation of the object.  
 A snapshot of the object gleaming in immaculate condition.  
 A photo showcasing the flawless details of the item.  
 A close-up shot revealing the perfect contours of the object.  
 An image displaying the object without any damage.  
 A photograph capturing the untouched elegance of the item.

## Anomaly Response

A close-up shot of a broken piece lying on the ground.  
 Zoomed-in view of fractured parts of an object.  
 An image showcasing the aftermath of impact.  
 A photo capturing the cracks and splinters on a surface.  
 Focus on the shattered fragments of the item.  
 Detail shot revealing the extent of the damage.  
 A picture showing the disarray caused by the breakage.  
 Close-up of the fractured edges of the object.  
 Macro image highlighting the fissures and fractures.  
 A snapshot displaying the fragmented remains.  
 A photograph depicting the visible signs of wear and tear.  
 An image illustrating the consequences of force.  
 Zoomed-in view of the compromised structure.  
 A close-up shot of the broken components.  
 Focus on the cracks spidering across the surface.  
 An image revealing the impact points of damage.  
 A photo displaying the shattered remnants scattered around.  
 A snapshot capturing the broken pieces in disarray.  
 A detailed shot showcasing the fractured edges.  
 A close-up view of the object's fragmented state.  
 Zoomed-in image revealing the intricate fractures.  
 A photograph showing the object's structural weakness.  
 An image highlighting the visible signs of breakage.  
 A close-up shot emphasizing the damage inflicted.  
 A picture displaying the fragmented parts separated.  
 An image illustrating the object's compromised integrity.  
 Focus on the fragmented surface texture.  
 A photo showcasing the fragmented pieces in detail.  
 A snapshot capturing the object's state of disrepair.  
 An image displaying the fractured sections.  
 A close-up shot revealing the cracks and splits.  
 Zoomed-in view showcasing the shattered components.  
 A photograph showing the fragmented elements strewn about.  
 An image illustrating the object's weakened structure.  
 A picture displaying the visible fractures and breaks.  
 A snapshot capturing the fragmented remnants.  
 A close-up shot highlighting the shattered fragments.  
 An image revealing the object's susceptibility to damage.  
 Focus on the broken parts scattered on the surface.  
 A photo showing the shattered pieces in close detail.  
 A snapshot capturing the object's state of deterioration.  
 A close-up shot displaying the cracks in intricate detail.  
 An image emphasizing the extent of the damage inflicted.  
 A photograph revealing the fractures along the surface.  
 Focus on the splintered sections of the object.  
 A picture showing the fragmented pieces in disarray.  
 An image highlighting the points of weakness.  
 A close-up shot of the broken segments.  
 A photo showcasing the fractured areas.  
 A snapshot revealing the cracks branching out.  
 An image illustrating the object's vulnerability to damage.  
 Focus on the shattered remnants strewn across.  
 A close-up shot capturing the fractured edges.  
 A photograph showing the object's susceptibility to breakage.  
 An image revealing the fragmented structure.  
 A picture displaying the broken components separated.  
 A snapshot capturing the object's state of disintegration.  
 A close-up shot highlighting the cracks and breaks.  
 An image showcasing the shattered fragments in detail.  
 Focus on the compromised sections of the object.  
 A photo displaying the fragmented pieces scattered.  
 A snapshot revealing the object's fragility.  
 A close-up shot of the object's damaged areas.  
 An image emphasizing the severity of the damage.  
 A photograph showcasing the fractured surface.  
 Focus on the shattered pieces lying on the ground.  
 A picture showing the fragmented parts dislodged.  
 An image illustrating the object's susceptibility to fractures.  
 A photo displaying the fragmented elements in close-up.  
 A snapshot revealing the object's weakened state.  
 An image highlighting the points of impact.  
 Focus on the shattered fragments dispersed around.  
 A close-up shot of the fractured surface texture.  
 A photograph showcasing the object's vulnerability.  
 An image revealing the extent of the breakage.  
 A picture displaying the broken pieces in detail.  
 A snapshot capturing the object's state of decay.  
 A close-up shot highlighting the fractures and splinters.  
 An image showcasing the shattered remnants in close detail.  
 Focus on the compromised integrity of the object.  
 A photo displaying the fragmented sections separated.  
 A snapshot revealing the object's state of disrepair.  
 A close-up shot capturing the cracks and splits.  
 An image illustrating the object's susceptibility to damage.  
 A photograph showing the fractured areas.  
 Focus on the splintered sections of the object.  
 A picture showcasing the fragmented pieces in disarray.  
 An image highlighting the points of weakness.  
 A close-up shot of the broken segments.  
 A photo revealing the cracks branching out.  
 A snapshot capturing the object's vulnerability to breakage.  
 An image emphasizing the extent of the damage inflicted.  
 Focus on the shattered remnants strewn across.  
 A close-up shot capturing the fractured edges.  
 A photograph revealing the object's vulnerability to breakage.  
 An image illustrating the fragmented structure.  
 A picture displaying the broken components separated.  
 A snapshot revealing the object's state of disintegration.

Figure 3: ChatGPT prompt ensemble 3

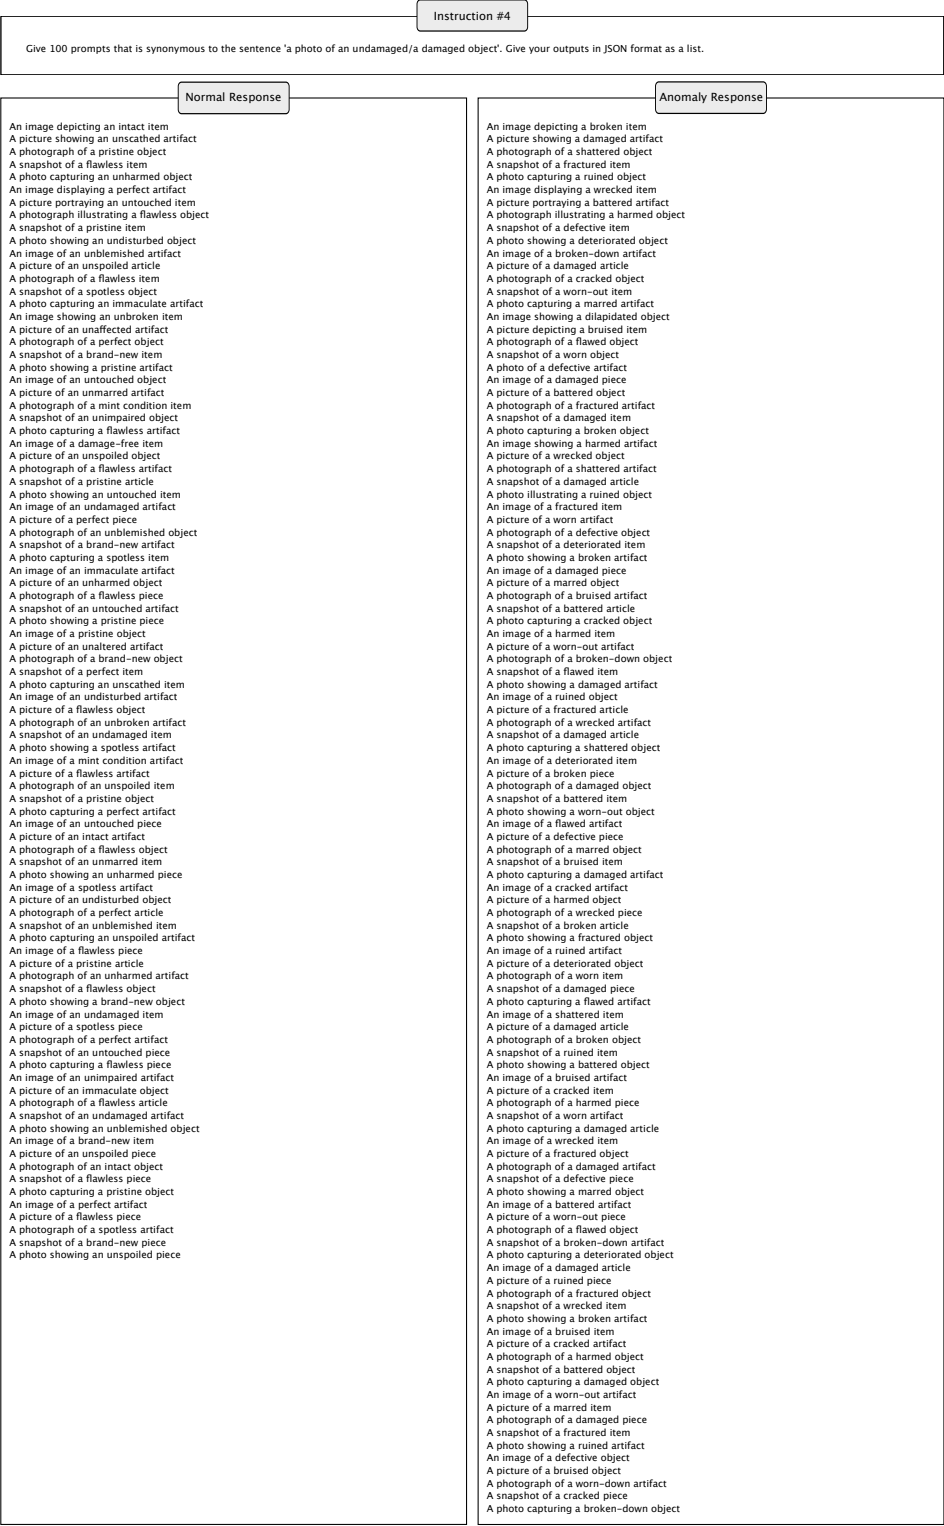

Figure 4: ChatGPT prompt ensemble 4

## Instruction #5

Give 100 prompts that describe a photo of an undamaged/a defective manufacturing object. Do not mention specific object name. Give your outputs in JSON format as a list.

## Normal Response

A close-up of a pristine surface on a manufacturing object.  
 An image showing a perfectly aligned component in a manufacturing object.  
 A photograph depicting a smoothly functioning mechanism within the manufacturing object.  
 A photo highlighting a flawlessly assembled manufacturing object.  
 A close-up shot revealing the impeccable material of the manufacturing object.  
 An overhead view of an intact section in the manufacturing object.  
 A detailed picture showing a spotless surface of the manufacturing object.  
 An image capturing a seamless connection point on the manufacturing object.  
 A photograph displaying a fully assembled part in the manufacturing object.  
 A close-up shot of a flawlessly sealed seam on the manufacturing object.  
 An overhead view of a pristine surface on the manufacturing object.  
 A detailed picture showing a well-maintained area of the manufacturing object.  
 An image depicting a perfectly welded joint in the manufacturing object.  
 A photograph revealing a smooth edge on the manufacturing object.  
 A close-up of a polished section in the manufacturing object.  
 An overhead view of a securely fastened part on the manufacturing object.  
 A detailed picture highlighting a flawlessly molded section of the manufacturing object.  
 An image displaying a perfectly finished surface on the manufacturing object.  
 A photograph showing a flawlessly smooth surface on the manufacturing object.  
 A close-up shot of a flawlessly crafted component in the manufacturing object.  
 An overhead view of a perfectly symmetrical section in the manufacturing object.  
 A detailed picture showing a perfectly labeled area of the manufacturing object.  
 An image capturing a flawlessly stamped section of the manufacturing object.  
 A photograph displaying a perfectly shaped surface on the manufacturing object.  
 A close-up of a flawlessly molded section in the manufacturing object.  
 An overhead view of a flawlessly engraved detail on the manufacturing object.  
 A detailed picture showing a perfectly coated surface of the manufacturing object.  
 An image depicting a perfectly calibrated component in the manufacturing object.  
 A photograph showing a flawlessly smooth surface on the manufacturing object.  
 A close-up shot of a flawlessly applied coating on the manufacturing object.  
 An overhead view of a perfectly machined section in the manufacturing object.  
 A detailed picture highlighting a flawlessly crafted detail on the manufacturing object.  
 An image capturing a perfectly shaped contour of the manufacturing object.  
 A photograph displaying a flawlessly painted surface on the manufacturing object.  
 A close-up of a flawlessly assembled joint in the manufacturing object.  
 An overhead view of a flawlessly designed section in the manufacturing object.  
 A detailed picture showing a perfectly casted component in the manufacturing object.  
 An image depicting a flawlessly extruded detail on the manufacturing object.  
 A photograph revealing a perfectly molded surface on the manufacturing object.  
 A close-up shot of a flawlessly formed part on the manufacturing object.  
 An overhead view of a flawlessly polished section in the manufacturing object.  
 A detailed picture highlighting a flawlessly machined detail on the manufacturing object.  
 An image capturing a perfectly formed contour of the manufacturing object.  
 A photograph displaying a flawlessly welded seam on the manufacturing object.  
 A close-up of a flawlessly stamped detail on the manufacturing object.  
 An overhead view of a flawlessly engraved area on the manufacturing object.  
 An image depicting a flawlessly calibrated component in the manufacturing object.  
 A photograph revealing a perfectly smooth surface on the manufacturing object.  
 A close-up shot of a flawlessly applied paint on the manufacturing object.  
 An overhead view of a flawlessly machined component in the manufacturing object.  
 A detailed picture highlighting a flawlessly crafted surface on the manufacturing object.  
 A photograph displaying a flawlessly polished surface on the manufacturing object.  
 A close-up of a flawlessly assembled joint in the manufacturing object.  
 An overhead view of a flawlessly designed section in the manufacturing object.  
 A detailed picture showing a perfectly casted component in the manufacturing object.  
 An image depicting a flawlessly extruded detail on the manufacturing object.  
 A photograph revealing a perfectly molded surface on the manufacturing object.  
 A close-up shot of a flawlessly formed part on the manufacturing object.  
 An overhead view of a flawlessly polished section in the manufacturing object.  
 A detailed picture highlighting a flawlessly machined detail on the manufacturing object.  
 An image capturing a perfectly formed contour of the manufacturing object.  
 A photograph displaying a flawlessly welded seam on the manufacturing object.  
 A close-up of a flawlessly stamped detail on the manufacturing object.  
 An overhead view of a flawlessly engraved area on the manufacturing object.  
 An image depicting a flawlessly calibrated component in the manufacturing object.  
 A photograph revealing a perfectly smooth surface on the manufacturing object.  
 A close-up shot of a flawlessly applied paint on the manufacturing object.  
 An overhead view of a flawlessly machined component in the manufacturing object.  
 A detailed picture highlighting a flawlessly crafted surface on the manufacturing object.  
 An image capturing a perfectly formed contour of the manufacturing object.

## Anomaly Response

A close-up of a cracked surface on a manufacturing object.  
 A photo showing a misaligned component in a manufacturing object.  
 An image depicting a broken mechanism within the manufacturing object.  
 A photograph highlighting a manufacturing defect due to improper assembly.  
 A close-up shot revealing a flaw in the material of the manufacturing object.  
 An overhead view of a warped section in the manufacturing object.  
 A detailed picture showing corrosion on the surface of the manufacturing object.  
 An image capturing a faulty connection point on the manufacturing object.  
 A photo displaying a missing part in the assembly of the manufacturing object.  
 A close-up shot of a seam failure on the manufacturing object.  
 An overhead view of a dent on the surface of the manufacturing object.  
 A detailed picture showing a leakage point in the manufacturing object.  
 An image revealing a defect in the welding of the manufacturing object.  
 A photograph showing a chipped edge on the manufacturing object.  
 A close-up of a bent section in the manufacturing object.  
 An overhead view of a dislodged component in the manufacturing object.  
 A photo capturing a scratch on the surface of the manufacturing object.  
 A detailed picture showing a manufacturing defect due to material fatigue.  
 An image depicting a bulge in the structure of the manufacturing object.  
 A photograph revealing a defect in the coating of the manufacturing object.  
 A close-up shot of a tear in the fabric of the manufacturing object.  
 An overhead view showing a loose fastening on the manufacturing object.  
 A detailed picture highlighting a flaw in the molding of the manufacturing object.  
 An image displaying a defect in the finishing of the manufacturing object.  
 A photograph showing a crackling surface on the manufacturing object.  
 A close-up shot revealing a faulty circuitry within the manufacturing object.  
 An overhead view of a discolored area on the manufacturing object.  
 A detailed picture showing a bulging seam on the manufacturing object.  
 An image depicting a distortion in the shape of the manufacturing object.  
 A photograph revealing a splintered edge on the manufacturing object.  
 A close-up of a frayed section in the manufacturing object.  
 An overhead view of a protruding part on the manufacturing object.  
 A detailed picture showing a defect in the labeling of the manufacturing object.  
 An image capturing a flaw in the stamping of the manufacturing object.  
 A photograph displaying a warped surface on the manufacturing object.  
 A close-up shot revealing an incomplete mold on the manufacturing object.  
 An overhead view of a cracked junction in the manufacturing object.  
 A detailed picture showing a defect in the engraving of the manufacturing object.  
 An image depicting a blister in the coating of the manufacturing object.  
 A photograph showing a peeling surface on the manufacturing object.  
 A close-up of a rusted section in the manufacturing object.  
 An overhead view of a malformed area on the manufacturing object.  
 A detailed picture showing a defect in the threading of the manufacturing object.  
 An image capturing a flaw in the calibration of the manufacturing object.  
 A photograph revealing a crack in the foundation of the manufacturing object.  
 A close-up shot of a detached component in the manufacturing object.  
 An overhead view of a punctured area on the manufacturing object.  
 A detailed picture showing a defect in the casting of the manufacturing object.  
 An image depicting a deformation in the structure of the manufacturing object.  
 A photograph showing a broken seal on the manufacturing object.  
 A close-up of a warped corner in the manufacturing object.  
 An overhead view of a flawed pattern on the manufacturing object.  
 A detailed picture showing a defect in the glazing of the manufacturing object.  
 An image capturing a flaw in the welding seam of the manufacturing object.  
 A photograph revealing a crack in the foundation of the manufacturing object.  
 A close-up shot of a detached component in the manufacturing object.  
 An overhead view of a punctured area on the manufacturing object.  
 A detailed picture showing a defect in the casting of the manufacturing object.  
 An image depicting a deformation in the structure of the manufacturing object.  
 A photograph showing a broken seal on the manufacturing object.  
 A close-up of a warped corner in the manufacturing object.  
 An overhead view of a flawed pattern on the manufacturing object.  
 A detailed picture showing a defect in the glazing of the manufacturing object.  
 An image capturing a flaw in the welding seam of the manufacturing object.  
 A photograph revealing a crack in the foundation of the manufacturing object.  
 A close-up shot of a detached component in the manufacturing object.  
 An overhead view of a punctured area on the manufacturing object.  
 A detailed picture showing a defect in the casting of the manufacturing object.  
 An image depicting a deformation in the structure of the manufacturing object.  
 A photograph showing a broken seal on the manufacturing object.  
 A close-up of a warped corner in the manufacturing object.  
 An overhead view of a flawed pattern on the manufacturing object.  
 A detailed picture showing a defect in the glazing of the manufacturing object.  
 An image capturing a flaw in the welding seam of the manufacturing object.

Figure 5: ChatGPT prompt ensemble 5

## 2 Combining language and vision guidance

Language- and vision-guided anomaly detection is complementary to each other. Combining their results can improve the overall AC and AS performance. Tab. 2 in the main paper shows the quantities that are combined under the different settings. In this section, we describe in detail how the aggregation is done. Tab. 1 shows the equations and parameter values that are used to combine the language- and vision-guided anomaly outputs under the zero-/few-shot settings for both the AC and AS tasks.

The aggregation involves two parameters  $\alpha$  and  $\beta$ . The values of the language- and vision-guided outputs are not directly comparable and exhibit very different ranges. We introduce  $\beta$  as a scaling factor that brings the values of the vision-guided outputs into the same range as that of the language-guided outputs. The value of  $\beta$  is determined approximately by visualising the histogram distributions of the anomaly scores for the language- and vision-guided outputs and then choosing a  $\beta$  value that roughly matches the two distributions to each other.  $\alpha$  is a weighting that controls the balance between language and vision guidance. We observe from our experiments that the anomaly detection performance is insensitive to the exact values of  $\alpha$  and  $\beta$  and an approximate choice of  $\alpha$  and  $\beta$  suffices.

| Task | Shot   | Aggregation                                          | $\alpha$ | $\beta$ |
|------|--------|------------------------------------------------------|----------|---------|
| AC   | 0-shot | $s^{lang}$                                           | -        | -       |
|      | k-shot | $(1 - \alpha)s^{lang} + (1 - \alpha)\beta s^{vis,k}$ | 0.5      | 3.5     |
| AS   | 0-shot | $(1 - \alpha)M^{lang} + (1 - \alpha)\beta M^{vis,0}$ | 0.5      | 80      |
|      | k-shot | $(1 - \alpha)M^{lang} + (1 - \alpha)\beta M^{vis,k}$ | 0.85     | 3.5     |

Table 1: Aggregation of language and vision guidance under different settings.

### 3 Detailed quantitative results

In this section, we report the performance breakdown of each object class for the evaluation metrics shown in Tab. 1 and 4 of the main paper. Tab. 2-7 report the results on MVTec-AD and Tab. 8-13 report the results on VisA.

| MVTec-AD (AC) | $K = 0$         |           | $K = 1$  |                 | $K = 2$  |                 | $K = 4$   |                 |
|---------------|-----------------|-----------|----------|-----------------|----------|-----------------|-----------|-----------------|
| AUROC         | WinCLIP         | FADE      | WinCLIP+ | FADE            | WinCLIP+ | FADE            | WinCLIP+  | FADE            |
| Bottle        | 99.2±0.0        | 97.7±0.0  | 98.2±0.9 | 99.3±0.1        | 99.3±0.3 | 99.4±0.3        | 99.3±0.4  | 99.8±0.4        |
| Cable         | 86.5±0.0        | 85.5±0.0  | 88.9±1.9 | 93.1±2.0        | 88.4±0.7 | 95.1±1.4        | 90.9±0.9  | 96.1±0.3        |
| Capsule       | 72.9±0.0        | 67.8±0.0  | 72.3±6.8 | 71.5±11.3       | 77.3±8.8 | 80.3±13.2       | 82.3±8.9  | 91.0±1.9        |
| Carpet        | 100.0±0.0       | 99.3±0.0  | 99.8±0.3 | 99.9±0.1        | 99.8±0.3 | 100.0±0.1       | 100.0±0.0 | 100.0±0.0       |
| Grid          | 98.8±0.0        | 99.4±0.0  | 99.5±0.3 | 98.8±1.4        | 99.4±0.2 | 99.0±0.8        | 99.6±0.1  | 98.6±0.7        |
| Hazelnut      | 93.9±0.0        | 92.6±0.0  | 97.5±1.4 | 97.3±1.2        | 98.3±0.7 | 97.6±0.6        | 98.4±0.4  | 97.8±0.7        |
| Leather       | 100.0±0.0       | 100.0±0.0 | 99.9±0.0 | 100.0±0.0       | 99.9±0.0 | 100.0±0.0       | 100.0±0.0 | 100.0±0.0       |
| Metal nut     | 97.1±0.0        | 95.5±0.0  | 98.7±0.8 | 99.0±0.2        | 99.4±0.2 | 99.2±0.2        | 99.5±0.2  | 99.3±0.2        |
| Pill          | 79.1±0.0        | 81.6±0.0  | 91.2±2.1 | 95.3±0.6        | 92.3±0.7 | 95.9±0.7        | 92.8±1.0  | 95.8±0.4        |
| Screw         | 83.3±0.0        | 74.9±0.0  | 86.4±0.9 | 75.9±5.1        | 86.0±2.1 | 82.0±3.2        | 87.9±1.2  | 82.3±3.9        |
| Tile          | 100.0±0.0       | 99.9±0.0  | 99.9±0.0 | 100.0±0.0       | 99.9±0.2 | 100.0±0.0       | 99.9±0.1  | 100.0±0.0       |
| Toothbrush    | 87.5±0.0        | 82.5±0.0  | 92.2±4.9 | 92.8±3.2        | 97.5±1.6 | 93.1±2.2        | 96.7±2.6  | 94.7±2.1        |
| Transistor    | 88.0±0.0        | 86.4±0.0  | 83.4±3.8 | 88.9±0.5        | 85.3±1.7 | 90.2±2.0        | 85.7±2.5  | 91.3±1.5        |
| Wood          | 99.4±0.0        | 96.7±0.0  | 99.9±0.1 | 99.1±0.3        | 99.9±0.1 | 99.3±0.4        | 99.8±0.3  | 99.4±0.2        |
| Zipper        | 91.5±0.0        | 90.5±0.0  | 88.8±5.9 | 97.7±1.2        | 94.0±1.4 | 97.5±1.0        | 94.5±0.5  | 97.9±1.7        |
| Mean          | <b>91.8±0.0</b> | 90.0±0.0  | 93.1±2.0 | <b>93.9±0.7</b> | 94.4±1.3 | <b>95.2±1.0</b> | 95.2±1.3  | <b>96.3±0.4</b> |

Table 2: Comparison of anomaly classification (AC) performance in terms of class-wise AUROC on MVTec-AD. We report the mean and standard deviation over 5 random seeds.

| MVTec-AD (AC) | $K = 0$         |           | $K = 1$   |                 | $K = 2$   |                 | $K = 4$   |                 |
|---------------|-----------------|-----------|-----------|-----------------|-----------|-----------------|-----------|-----------------|
| AUPR          | WinCLIP         | FADE      | WinCLIP+  | FADE            | WinCLIP+  | FADE            | WinCLIP+  | FADE            |
| Bottle        | 99.8±0.0        | 99.3±0.0  | 99.4±0.3  | 99.8±0.0        | 99.8±0.1  | 99.8±0.1        | 99.8±0.1  | 99.9±0.1        |
| Cable         | 91.2±0.0        | 90.4±0.0  | 93.2±1.1  | 95.6±1.6        | 92.9±0.6  | 97.2±1.1        | 94.4±0.3  | 97.8±0.1        |
| Capsule       | 91.5±0.0        | 90.0±0.0  | 91.6±2.7  | 89.7±4.8        | 93.3±3.6  | 93.7±5.6        | 95.1±3.3  | 97.9±0.4        |
| Carpet        | 100.0±0.0       | 99.8±0.0  | 99.9±0.1  | 100.0±0.0       | 99.9±0.1  | 100.0±0.0       | 100.0±0.0 | 100.0±0.0       |
| Grid          | 99.6±0.0        | 99.8±0.0  | 99.9±0.1  | 99.6±0.4        | 99.8±0.1  | 99.6±0.3        | 99.9±0.0  | 99.5±0.2        |
| Hazelnut      | 96.9±0.0        | 96.2±0.0  | 98.6±0.7  | 98.6±0.6        | 99.1±0.4  | 98.8±0.3        | 99.1±0.2  | 98.9±0.4        |
| Leather       | 100.0±0.0       | 100.0±0.0 | 100.0±0.0 | 100.0±0.0       | 100.0±0.0 | 100.0±0.0       | 100.0±0.0 | 100.0±0.0       |
| Metal nut     | 99.3±0.0        | 98.9±0.0  | 99.7±0.2  | 99.8±0.0        | 99.9±0.0  | 99.8±0.0        | 99.9±0.1  | 99.9±0.0        |
| Pill          | 95.7±0.0        | 96.4±0.0  | 98.3±0.5  | 99.1±0.1        | 98.6±0.1  | 99.3±0.1        | 98.6±0.2  | 99.2±0.1        |
| Screw         | 93.1±0.0        | 89.8±0.0  | 94.2±0.6  | 88.1±3.5        | 94.1±1.5  | 92.1±2.2        | 94.9±0.8  | 91.9±2.9        |
| Tile          | 100.0±0.0       | 100.0±0.0 | 100.0±0.0 | 100.0±0.0       | 100.0±0.1 | 100.0±0.0       | 100.0±0.0 | 100.0±0.0       |
| Toothbrush    | 95.6±0.0        | 93.3±0.0  | 96.7±2.0  | 97.3±1.2        | 99.0±0.6  | 97.4±0.9        | 98.7±1.1  | 98.0±0.8        |
| Transistor    | 87.1±0.0        | 83.6±0.0  | 79.0±4.0  | 85.9±0.4        | 80.7±2.3  | 87.7±1.9        | 80.7±3.2  | 88.9±1.9        |
| Wood          | 99.5±0.0        | 99.0±0.0  | 100.0±0.0 | 99.7±0.1        | 100.0±0.0 | 99.8±0.1        | 99.9±0.1  | 99.8±0.1        |
| Zipper        | 97.8±0.0        | 97.2±0.0  | 96.8±1.8  | 99.3±0.4        | 98.3±0.4  | 99.3±0.3        | 99.5±0.2  | 99.4±0.5        |
| Mean          | <b>96.5±0.0</b> | 95.6±0.0  | 96.5±0.9  | <b>96.8±0.3</b> | 97.0±0.7  | <b>97.6±0.5</b> | 97.3±0.6  | <b>98.1±0.2</b> |

Table 3: Comparison of anomaly classification (AC) performance in terms of class-wise AUPR on MVTec-AD. We report the mean and standard deviation over 5 random seeds.

| MVTec-AD (AC) | $K = 0$         |           | $K = 1$  |                 | $K = 2$  |                 | $K = 4$  |                 |
|---------------|-----------------|-----------|----------|-----------------|----------|-----------------|----------|-----------------|
| $F_1$ -max    | WinCLIP         | FADE      | WinCLIP+ | FADE            | WinCLIP+ | FADE            | WinCLIP+ | FADE            |
| Bottle        | 97.6±0.0        | 96.1±0.0  | 96.5±1.3 | 98.4±0.0        | 97.7±0.7 | 98.3±0.7        | 97.8±0.6 | 98.9±1.2        |
| Cable         | 84.5±0.0        | 86.2±0.0  | 86.1±1.3 | 90.2±1.6        | 85.2±0.7 | 91.4±1.7        | 87.2±0.6 | 92.6±0.8        |
| Capsule       | 91.4±0.0        | 93.0±0.0  | 91.6±0.7 | 93.2±0.8        | 92.1±0.7 | 93.5±1.3        | 92.5±0.5 | 94.5±1.0        |
| Carpet        | 99.4±0.0        | 97.8±0.0  | 99.2±0.8 | 99.7±0.3        | 99.3±0.7 | 99.8±0.3        | 99.9±0.2 | 99.7±0.3        |
| Grid          | 98.2±0.0        | 98.2±0.0  | 98.9±0.4 | 98.4±1.2        | 99.1±0.0 | 97.7±1.6        | 99.1±0.0 | 97.3±1.1        |
| Hazelnut      | 89.7±0.0        | 88.6±0.0  | 94.7±2.3 | 94.4±1.8        | 95.6±1.6 | 94.3±1.3        | 96.2±1.0 | 95.0±0.9        |
| Leather       | 100.0±0.0       | 100.0±0.0 | 99.5±0.0 | 100.0±0.0       | 99.7±0.2 | 100.0±0.0       | 99.8±0.2 | 100.0±0.0       |
| Metal nut     | 96.3±0.0        | 95.1±0.0  | 97.7±1.0 | 98.5±0.6        | 98.4±0.5 | 98.7±0.3        | 98.5±0.6 | 99.2±0.3        |
| Pill          | 91.6±0.0        | 91.6±0.0  | 93.8±0.7 | 95.3±0.5        | 94.3±0.4 | 95.4±0.5        | 94.1±0.4 | 95.3±0.4        |
| Screw         | 87.4±0.0        | 86.1±0.0  | 88.5±0.3 | 87.4±0.9        | 89.0±0.6 | 87.9±1.0        | 89.6±0.7 | 88.4±1.2        |
| Tile          | 99.9±0.0        | 99.4±0.0  | 98.9±0.2 | 99.9±0.3        | 99.2±0.3 | 100.0±0.0       | 99.2±0.3 | 100.0±0.0       |
| Toothbrush    | 87.9±0.0        | 87.5±0.0  | 94.1±1.9 | 92.1±2.6        | 96.7±1.8 | 91.7±2.7        | 96.8±2.3 | 93.0±2.6        |
| Transistor    | 79.5±0.0        | 78.3±0.0  | 75.1±3.1 | 78.6±0.8        | 75.9±2.4 | 81.2±3.0        | 76.6±2.8 | 82.8±2.9        |
| Wood          | 98.3±0.0        | 95.2±0.0  | 99.4±0.3 | 97.7±0.7        | 99.5±0.4 | 98.3±0.6        | 99.2±0.9 | 98.2±0.4        |
| Zipper        | 92.9±0.0        | 92.7±0.0  | 92.1±2.5 | 97.6±1.1        | 94.4±0.3 | 96.9±0.7        | 94.7±0.4 | 97.6±1.1        |
| Mean          | <b>92.9±0.0</b> | 92.4±0.0  | 93.7±1.1 | <b>94.8±0.2</b> | 94.4±0.8 | <b>95.0±0.4</b> | 94.7±0.8 | <b>95.5±0.4</b> |

Table 4: Comparison of anomaly classification (AC) performance in terms of class-wise  $F_1$ -max on MVTec-AD. We report the mean and standard deviation over 5 random seeds.

| MVTec-AD (AS) | $K = 0$  |                 | $K = 1$  |                 | $K = 2$         |          | $K = 4$         |                 |
|---------------|----------|-----------------|----------|-----------------|-----------------|----------|-----------------|-----------------|
|               | WinCLIP  | FADE            | WinCLIP+ | FADE            | WinCLIP+        | FADE     | WinCLIP+        | FADE            |
| Bottle        | 89.5±0.0 | 89.7±0.0        | 97.5±0.2 | 96.4±0.3        | 97.7±0.1        | 96.7±0.2 | 97.8±0.0        | 96.7±0.3        |
| Cable         | 77.0±0.0 | 80.1±0.0        | 93.8±0.6 | 94.0±0.3        | 94.3±0.4        | 94.4±0.4 | 94.9±0.1        | 94.8±0.2        |
| Capsule       | 86.9±0.0 | 89.5±0.0        | 94.6±0.8 | 97.0±0.5        | 96.4±0.3        | 97.6±0.7 | 96.2±0.5        | 98.2±0.1        |
| Carpet        | 95.4±0.0 | 99.3±0.0        | 99.4±0.0 | 99.4±0.1        | 99.3±0.0        | 99.4±0.0 | 99.3±0.0        | 99.4±0.0        |
| Grid          | 82.2±0.0 | 98.4±0.0        | 96.8±1.0 | 96.1±1.1        | 97.7±0.8        | 96.2±0.7 | 98.0±0.2        | 96.7±0.7        |
| Hazelnut      | 94.3±0.0 | 97.1±0.0        | 98.5±0.2 | 99.2±0.2        | 98.7±0.1        | 99.3±0.2 | 98.8±0.0        | 99.4±0.1        |
| Leather       | 96.7±0.0 | 99.2±0.0        | 99.3±0.0 | 99.4±0.0        | 99.3±0.0        | 99.4±0.0 | 99.3±0.0        | 99.4±0.0        |
| Metal nut     | 61.0±0.0 | 65.5±0.0        | 90.0±0.6 | 91.6±0.6        | 91.4±0.4        | 92.4±0.9 | 92.9±0.4        | 93.7±1.0        |
| Pill          | 80.0±0.0 | 84.4±0.0        | 96.4±0.3 | 96.2±0.7        | 97.0±0.2        | 96.7±0.2 | 97.1±0.0        | 96.8±0.2        |
| Screw         | 89.6±0.0 | 97.9±0.0        | 94.5±0.4 | 96.2±0.8        | 95.2±0.3        | 96.6±1.0 | 96.0±0.5        | 96.6±1.0        |
| Tile          | 77.6±0.0 | 92.7±0.0        | 96.3±0.2 | 93.7±0.3        | 96.5±0.1        | 93.9±0.3 | 96.6±0.1        | 93.8±0.2        |
| Toothbrush    | 86.9±0.0 | 90.8±0.0        | 97.8±0.1 | 98.6±0.3        | 98.1±0.1        | 98.8±0.2 | 98.4±0.5        | 99.0±0.1        |
| Transistor    | 74.7±0.0 | 62.8±0.0        | 85.0±1.8 | 82.8±3.3        | 88.3±1.0        | 85.7±2.2 | 88.5±1.2        | 88.5±1.3        |
| Wood          | 93.4±0.0 | 97.1±0.0        | 94.6±1.0 | 95.0±0.8        | 95.3±0.4        | 95.3±0.3 | 95.4±0.2        | 95.3±0.2        |
| Zipper        | 91.6±0.0 | 95.0±0.0        | 93.9±0.8 | 94.9±0.5        | 94.1±0.7        | 94.3±0.2 | 94.2±0.4        | 94.4±0.1        |
| Mean          | 85.1±0.0 | <b>89.6±0.0</b> | 95.2±0.5 | <b>95.4±0.3</b> | <b>96.0±0.3</b> | 95.8±0.2 | <b>96.2±0.3</b> | <b>96.2±0.1</b> |

Table 5: Comparison of anomaly segmentation (AS) performance in terms of class-wise pixel-AUROC on MVTec-AD. We report the mean and standard deviation over 5 random seeds.

| MVTec-AD (AS) | $K = 0$  |                 | $K = 1$  |                 | $K = 2$  |                 | $K = 4$  |                 |
|---------------|----------|-----------------|----------|-----------------|----------|-----------------|----------|-----------------|
|               | WinCLIP  | FADE            | WinCLIP+ | FADE            | WinCLIP+ | FADE            | WinCLIP+ | FADE            |
| PRO           |          |                 |          |                 |          |                 |          |                 |
| Bottle        | 76.4±0.0 | 80.3±0.0        | 91.2±0.4 | 89.1±0.7        | 91.8±0.3 | 89.2±0.3        | 91.6±0.2 | 89.3±0.4        |
| Cable         | 42.9±0.0 | 68.1±0.0        | 72.5±2.3 | 84.4±0.4        | 74.7±2.3 | 85.9±0.4        | 77.0±1.1 | 87.1±0.4        |
| Capsule       | 62.1±0.0 | 86.1±0.0        | 85.6±2.7 | 92.2±1.4        | 90.6±0.6 | 93.9±2.1        | 90.1±1.5 | 95.6±0.2        |
| Carpet        | 84.1±0.0 | 98.0±0.0        | 97.4±0.4 | 97.7±0.2        | 97.3±0.3 | 97.6±0.3        | 97.0±0.2 | 97.5±0.1        |
| Grid          | 57.0±0.0 | 84.8±0.0        | 90.5±2.7 | 89.7±2.2        | 92.8±2.5 | 89.8±1.3        | 93.6±0.6 | 90.7±1.9        |
| Hazelnut      | 81.6±0.0 | 92.6±0.0        | 93.7±0.9 | 94.4±1.0        | 94.2±0.3 | 95.0±0.9        | 94.2±0.3 | 95.5±0.6        |
| Leather       | 91.1±0.0 | 98.2±0.0        | 98.6±0.0 | 98.6±0.3        | 98.3±0.4 | 98.5±0.2        | 98.0±0.4 | 98.1±0.3        |
| Metal nut     | 31.8±0.0 | 69.2±0.0        | 84.7±1.1 | 87.3±0.6        | 86.7±0.8 | 88.1±1.0        | 89.4±0.1 | 89.7±1.1        |
| Pill          | 65.0±0.0 | 84.4±0.0        | 93.5±0.2 | 94.8±0.3        | 94.5±0.2 | 95.0±0.2        | 94.6±0.3 | 95.1±0.1        |
| Screw         | 68.5±0.0 | 91.5±0.0        | 82.3±1.1 | 85.7±2.0        | 84.1±0.5 | 87.5±2.8        | 86.3±1.8 | 87.5±3.1        |
| Tile          | 51.2±0.0 | 80.6±0.0        | 89.4±0.4 | 82.1±1.0        | 89.6±0.4 | 82.5±0.6        | 89.9±0.3 | 82.3±0.6        |
| Toothbrush    | 67.7±0.0 | 89.7±0.0        | 85.3±1.0 | 86.8±2.0        | 84.7±1.4 | 88.6±1.1        | 86.0±3.3 | 89.7±1.0        |
| Transistor    | 43.4±0.0 | 55.1±0.0        | 65.0±1.8 | 65.4±2.7        | 68.6±1.1 | 67.8±1.4        | 69.0±1.1 | 71.3±1.4        |
| Wood          | 74.1±0.0 | 91.7±0.0        | 91.0±0.6 | 88.4±1.1        | 91.8±0.6 | 87.6±2.4        | 91.7±0.3 | 86.1±1.7        |
| Zipper        | 71.7±0.0 | 87.5±0.0        | 86.0±1.7 | 87.7±0.7        | 86.4±1.6 | 86.4±0.3        | 86.9±0.7 | 86.6±0.3        |
| Mean          | 64.6±0.0 | <b>84.5±0.0</b> | 87.1±1.2 | <b>88.3±0.3</b> | 88.4±0.9 | <b>88.9±0.2</b> | 89.0±0.8 | <b>89.5±0.2</b> |

Table 6: Comparison of anomaly segmentation (AS) performance in terms of class-wise PRO on MVTec-AD. We report the mean and standard deviation over 5 random seeds.

| MVTec-AD (AS) | $K = 0$  |                 | $K = 1$         |          | $K = 2$         |          | $K = 4$         |          |
|---------------|----------|-----------------|-----------------|----------|-----------------|----------|-----------------|----------|
|               | WinCLIP  | FADE            | WinCLIP+        | FADE     | WinCLIP+        | FADE     | WinCLIP+        | FADE     |
| $F_1$ -max    |          |                 |                 |          |                 |          |                 |          |
| Bottle        | 58.1±0.0 | 50.8±0.0        | 72.8±0.8        | 67.5±1.2 | 73.2±0.9        | 68.0±0.6 | 73.3±0.6        | 67.9±0.9 |
| Cable         | 19.7±0.0 | 20.5±0.0        | 49.4±3.3        | 53.5±1.4 | 51.2±1.3        | 55.4±0.7 | 54.7±1.1        | 56.7±1.1 |
| Capsule       | 21.7±0.0 | 21.7±0.0        | 29.7±7.8        | 30.0±6.9 | 43.5±1.4        | 36.6±9.3 | 40.7±4.9        | 43.9±0.7 |
| Carpet        | 49.7±0.0 | 72.3±0.0        | 73.3±1.5        | 72.1±0.6 | 72.9±1.3        | 71.8±0.8 | 72.0±0.7        | 71.3±0.6 |
| Grid          | 18.6±0.0 | 46.4±0.0        | 50.7±4.5        | 42.1±4.1 | 53.4±3.8        | 41.5±2.7 | 52.7±1.5        | 41.4±2.8 |
| Hazelnut      | 37.6±0.0 | 45.4±0.0        | 68.9±2.6        | 72.7±3.7 | 70.5±1.7        | 74.2±3.8 | 71.0±0.3        | 76.0±1.1 |
| Leather       | 39.7±0.0 | 50.2±0.0        | 58.0±0.7        | 59.9±2.3 | 57.5±0.6        | 58.9±1.7 | 56.3±1.0        | 57.3±1.5 |
| Metal nut     | 32.4±0.0 | 30.1±0.0        | 59.4±1.7        | 61.5±2.2 | 62.7±1.5        | 64.1±3.1 | 67.4±1.6        | 68.4±3.4 |
| Pill          | 17.6±0.0 | 21.3±0.0        | 64.7±1.8        | 64.0±1.7 | 67.8±0.5        | 65.9±0.8 | 67.9±0.4        | 67.0±0.8 |
| Screw         | 13.5±0.0 | 25.8±0.0        | 22.2±2.8        | 16.7±3.7 | 22.4±2.8        | 19.5±6.0 | 30.1±4.3        | 19.0±8.5 |
| Tile          | 32.6±0.0 | 56.4±0.0        | 71.2±0.4        | 58.8±1.2 | 71.9±0.6        | 59.1±1.1 | 72.2±0.6        | 58.9±0.8 |
| Toothbrush    | 17.1±0.0 | 23.2±0.0        | 62.7±3.6        | 63.5±5.7 | 65.8±2.2        | 63.6±3.7 | 69.4±4.6        | 66.2±2.8 |
| Transistor    | 30.5±0.0 | 19.6±0.0        | 39.1±3.5        | 39.6±2.7 | 45.6±2.3        | 43.1±1.4 | 46.6±2.2        | 46.2±1.3 |
| Wood          | 51.5±0.0 | 67.2±0.0        | 65.2±1.4        | 63.9±1.0 | 65.8±0.6        | 63.7±0.8 | 65.1±0.5        | 63.4±0.9 |
| Zipper        | 34.4±0.0 | 46.5±0.0        | 50.6±3.9        | 53.0±1.2 | 50.9±4.5        | 51.8±1.1 | 52.8±2.7        | 52.0±1.3 |
| Mean          | 31.7±0.0 | <b>39.8±0.0</b> | <b>55.9±2.7</b> | 54.6±1.1 | <b>58.4±1.7</b> | 55.8±1.0 | <b>59.5±1.8</b> | 57.0±0.8 |

Table 7: Comparison of anomaly segmentation (AS) performance in terms of class-wise  $F_1$ -max on MVTec-AD. We report the mean and standard deviation over 5 random seeds.

| VisA (AC)  | $K = 0$         |          | $K = 1$   |                 | $K = 2$  |                 | $K = 4$  |                 |
|------------|-----------------|----------|-----------|-----------------|----------|-----------------|----------|-----------------|
|            | WinCLIP         | FADE     | WinCLIP+  | FADE            | WinCLIP+ | FADE            | WinCLIP+ | FADE            |
| AUROC      |                 |          |           |                 |          |                 |          |                 |
| Candle     | 95.4±0.0        | 94.7±0.0 | 93.4±1.4  | 95.7±1.6        | 94.8±1.0 | 96.3±0.8        | 95.1±0.3 | 96.6±0.6        |
| Capsules   | 85.0±0.0        | 79.8±0.0 | 85.0±3.1  | 83.8±1.7        | 84.9±0.8 | 84.9±1.8        | 86.8±1.7 | 85.3±1.7        |
| Cashew     | 92.1±0.0        | 91.6±0.0 | 94.0±0.4  | 94.1±1.1        | 94.3±0.5 | 94.8±0.6        | 95.2±0.8 | 95.4±0.7        |
| Chewinggum | 96.5±0.0        | 95.4±0.0 | 97.6±0.8  | 97.5±0.6        | 97.3±0.8 | 98.0±0.3        | 97.7±0.3 | 98.2±0.4        |
| Fryum      | 80.3±0.0        | 73.8±0.0 | 88.5±1.9  | 93.3±1.4        | 90.5±0.4 | 94.0±0.8        | 90.8±0.5 | 95.1±0.2        |
| Macaroni1  | 76.2±0.0        | 78.4±0.0 | 82.9±1.5  | 90.7±3.4        | 83.3±1.9 | 93.5±1.5        | 85.2±0.9 | 93.2±0.6        |
| Macaroni2  | 63.7±0.0        | 66.9±0.0 | 70.2±0.9  | 70.3±4.8        | 71.8±2.0 | 71.2±3.6        | 70.9±2.2 | 74.7±2.3        |
| PCB1       | 73.6±0.0        | 73.0±0.0 | 75.6±23.0 | 88.8±2.6        | 76.7±5.2 | 88.4±2.3        | 88.3±1.7 | 91.0±1.9        |
| PCB2       | 51.2±0.0        | 46.8±0.0 | 62.2±3.9  | 73.6±2.0        | 62.6±3.7 | 76.7±1.5        | 67.5±2.6 | 80.7±0.6        |
| PCB3       | 73.4±0.0        | 64.6±0.0 | 74.1±1.1  | 78.3±5.8        | 78.8±1.9 | 82.6±2.3        | 83.3±1.7 | 86.3±2.6        |
| PCB4       | 79.6±0.0        | 75.4±0.0 | 85.2±8.9  | 79.4±24.8       | 82.3±9.9 | 93.5±3.4        | 87.6±8.0 | 95.4±0.5        |
| Pipe fryum | 69.7±0.0        | 67.2±0.0 | 97.2±1.1  | 95.2±3.7        | 98.0±0.6 | 96.1±2.6        | 98.5±0.4 | 96.8±1.0        |
| Mean       | <b>78.1±0.0</b> | 75.6±0.0 | 83.8±4.0  | <b>86.7±2.0</b> | 84.6±2.4 | <b>89.2±0.4</b> | 87.3±1.8 | <b>90.7±0.3</b> |

Table 8: Comparison of anomaly classification (AC) performance in terms of class-wise AUROC on VisA. We report the mean and standard deviation over 5 random seeds.

| VisA (AC)  | $K = 0$         |          | $K = 1$   |                 | $K = 2$   |                 | $K = 4$  |                 |
|------------|-----------------|----------|-----------|-----------------|-----------|-----------------|----------|-----------------|
|            | WinCLIP         | FADE     | WinCLIP+  | FADE            | WinCLIP+  | FADE            | WinCLIP+ | FADE            |
| AUPR       |                 |          |           |                 |           |                 |          |                 |
| Candle     | 95.8±0.0        | 95.4±0.0 | 93.6±1.5  | 96.1±1.3        | 95.1±1.1  | 96.6±0.7        | 95.3±0.4 | 97.0±0.7        |
| Capsules   | 90.9±0.0        | 87.9±0.0 | 89.9±2.5  | 89.7±1.1        | 88.9±0.7  | 90.5±1.3        | 91.5±1.4 | 91.2±1.2        |
| Cashew     | 96.4±0.0        | 96.1±0.0 | 97.2±0.2  | 97.2±0.6        | 97.3±0.2  | 97.5±0.3        | 97.7±0.4 | 97.8±0.3        |
| Chewinggum | 98.6±0.0        | 98.0±0.0 | 99.0±0.3  | 99.0±0.2        | 98.9±0.3  | 99.2±0.2        | 99.0±0.1 | 99.2±0.2        |
| Fryum      | 90.1±0.0        | 87.0±0.0 | 94.7±1.0  | 97.0±0.7        | 95.8±0.2  | 97.3±0.4        | 96.0±0.3 | 97.9±0.1        |
| Macaroni1  | 75.8±0.0        | 79.0±0.0 | 84.9±1.2  | 92.2±2.2        | 84.7±1.5  | 94.2±1.1        | 86.5±0.6 | 94.0±0.4        |
| Macaroni2  | 60.3±0.0        | 64.9±0.0 | 68.4±1.8  | 69.6±4.5        | 70.4±1.8  | 69.8±3.4        | 69.6±2.8 | 73.4±2.5        |
| PCB1       | 78.4±0.0        | 73.5±0.0 | 76.5±19.0 | 87.4±3.6        | 78.3±4.3  | 87.3±3.2        | 87.7±1.7 | 90.7±2.7        |
| PCB2       | 49.2±0.0        | 45.3±0.0 | 64.9±3.3  | 73.1±1.7        | 65.8±4.0  | 76.9±1.9        | 71.3±3.4 | 81.3±0.9        |
| PCB3       | 76.5±0.0        | 63.9±0.0 | 73.5±1.6  | 79.8±5.3        | 80.9±1.6  | 84.2±2.6        | 84.8±1.8 | 87.8±2.8        |
| PCB4       | 77.7±0.0        | 69.1±0.0 | 78.5±15.5 | 76.1±21.7       | 72.5±16.2 | 90.7±3.4        | 85.6±8.9 | 93.5±1.3        |
| Pipe fryum | 82.3±0.0        | 81.6±0.0 | 98.6±0.5  | 97.4±2.1        | 99.0±0.3  | 98.0±1.4        | 99.2±0.2 | 98.4±0.5        |
| Mean       | <b>81.2±0.0</b> | 78.5±0.0 | 85.1±4.0  | <b>87.9±1.5</b> | 85.8±2.7  | <b>90.2±0.2</b> | 88.8±1.8 | <b>91.9±0.4</b> |

Table 9: Comparison of anomaly classification (AC) performance in terms of class-wise AUPR on VisA. We report the mean and standard deviation over 5 random seeds.

| VisA (AC)  | $K = 0$         |          | $K = 1$  |                 | $K = 2$  |                 | $K = 4$  |                 |
|------------|-----------------|----------|----------|-----------------|----------|-----------------|----------|-----------------|
|            | WinCLIP         | FADE     | WinCLIP+ | FADE            | WinCLIP+ | FADE            | WinCLIP+ | FADE            |
| $F_1$ -max |                 |          |          |                 |          |                 |          |                 |
| Candle     | 89.4±0.0        | 90.5±0.0 | 87.8±1.2 | 89.3±2.3        | 89.1±1.3 | 90.5±1.9        | 88.9±1.0 | 90.3±1.7        |
| Capsules   | 83.9±0.0        | 82.0±0.0 | 84.9±2.0 | 84.0±1.4        | 85.4±0.6 | 84.1±0.9        | 86.0±0.9 | 84.2±1.3        |
| Cashew     | 88.4±0.0        | 89.8±0.0 | 90.7±0.7 | 90.8±0.9        | 90.9±0.7 | 91.8±0.8        | 91.6±1.3 | 92.2±1.4        |
| Chewinggum | 94.8±0.0        | 92.6±0.0 | 95.6±0.9 | 95.7±0.6        | 95.4±0.6 | 96.0±0.8        | 95.7±0.5 | 96.3±0.6        |
| Fryum      | 82.7±0.0        | 80.2±0.0 | 87.2±1.4 | 91.3±2.0        | 88.4±0.6 | 91.4±1.2        | 88.9±0.8 | 92.6±0.3        |
| Macaroni1  | 74.2±0.0        | 74.9±0.0 | 76.2±1.4 | 83.6±2.8        | 76.7±2.0 | 86.2±2.3        | 78.2±1.2 | 85.8±0.9        |
| Macaroni2  | 69.8±0.0        | 69.0±0.0 | 72.3±1.1 | 71.1±2.2        | 73.9±0.9 | 71.5±2.7        | 73.1±1.6 | 72.8±1.6        |
| PCB1       | 71.0±0.0        | 72.2±0.0 | 81.3±6.6 | 85.1±0.6        | 73.2±3.7 | 84.3±1.7        | 83.1±2.2 | 86.0±1.7        |
| PCB2       | 67.1±0.0        | 67.4±0.0 | 67.2±0.3 | 72.9±2.0        | 67.3±0.3 | 73.7±0.9        | 67.7±0.6 | 76.1±1.4        |
| PCB3       | 71.0±0.0        | 67.8±0.0 | 73.5±1.5 | 74.9±3.5        | 73.9±1.3 | 76.6±2.5        | 77.0±1.4 | 80.1±2.3        |
| PCB4       | 74.9±0.0        | 76.6±0.0 | 86.1±2.1 | 84.6±10.3       | 86.8±3.8 | 90.5±3.7        | 84.6±7.0 | 93.1±1.2        |
| Pipe fryum | 80.7±0.0        | 81.0±0.0 | 94.4±0.7 | 93.8±2.2        | 95.4±0.8 | 94.5±2.2        | 95.6±0.7 | 94.4±1.6        |
| Mean       | <b>79.0±0.0</b> | 78.6±0.0 | 83.1±1.7 | <b>84.7±0.8</b> | 83.0±1.4 | <b>85.9±0.6</b> | 84.2±1.6 | <b>87.0±0.2</b> |

Table 10: Comparison of anomaly classification (AC) performance in terms of class-wise  $F_1$ -max on VisA. We report the mean and standard deviation over 5 random seeds.

| VisA (AS)  | $K = 0$  |                 | $K = 1$  |                 | $K = 2$  |                 | $K = 4$  |                 |
|------------|----------|-----------------|----------|-----------------|----------|-----------------|----------|-----------------|
|            | WinCLIP  | FADE            | WinCLIP+ | FADE            | WinCLIP+ | FADE            | WinCLIP+ | FADE            |
| Candle     | 88.9±0.0 | 93.0±0.0        | 97.4±0.2 | 98.4±0.1        | 97.7±0.1 | 98.5±0.1        | 97.8±0.2 | 98.5±0.1        |
| Capsules   | 81.6±0.0 | 80.8±0.0        | 96.4±0.6 | 95.4±0.4        | 96.8±0.3 | 96.0±0.3        | 97.1±0.2 | 96.3±0.4        |
| Cashew     | 84.7±0.0 | 89.2±0.0        | 98.5±0.2 | 99.0±0.1        | 98.5±0.1 | 99.0±0.1        | 98.7±0.0 | 99.0±0.1        |
| Chewinggum | 93.3±0.0 | 99.1±0.0        | 98.6±0.1 | 98.9±0.0        | 98.6±0.1 | 98.9±0.0        | 98.5±0.1 | 98.8±0.0        |
| Fryum      | 88.5±0.0 | 94.0±0.0        | 96.4±0.3 | 96.7±0.2        | 97.0±0.2 | 96.8±0.2        | 97.1±0.1 | 97.1±0.2        |
| Macaroni1  | 70.9±0.0 | 98.4±0.0        | 96.4±0.6 | 98.8±0.6        | 96.5±0.7 | 99.3±0.0        | 97.0±0.2 | 99.3±0.1        |
| Macaroni2  | 59.3±0.0 | 97.4±0.0        | 96.8±0.4 | 95.7±1.4        | 96.8±0.6 | 96.4±0.9        | 97.3±0.3 | 97.0±0.5        |
| PCB1       | 61.2±0.0 | 85.7±0.0        | 96.6±0.6 | 98.9±0.1        | 97.0±0.9 | 98.9±0.1        | 98.1±0.9 | 99.1±0.1        |
| PCB2       | 71.6±0.0 | 87.3±0.0        | 93.0±0.4 | 97.7±0.3        | 93.9±0.2 | 98.1±0.1        | 94.6±0.4 | 98.5±0.1        |
| PCB3       | 85.3±0.0 | 87.4±0.0        | 94.3±0.3 | 95.6±0.2        | 95.1±0.2 | 96.4±0.1        | 95.8±0.1 | 97.0±0.1        |
| PCB4       | 94.4±0.0 | 88.9±0.0        | 94.0±0.9 | 95.3±1.1        | 95.6±0.3 | 96.1±0.6        | 96.1±0.3 | 96.6±0.3        |
| Pipe fryum | 75.4±0.0 | 96.7±0.0        | 98.3±0.2 | 99.3±0.2        | 98.5±0.2 | 99.3±0.1        | 98.7±0.1 | 99.3±0.1        |
| Mean       | 79.6±0.0 | <b>91.5±0.0</b> | 96.4±0.4 | <b>97.5±0.1</b> | 96.8±0.3 | <b>97.8±0.1</b> | 97.2±0.2 | <b>98.0±0.0</b> |

Table 11: Comparison of anomaly segmentation (AS) performance in terms of class-wise pixel-AUROC on VisA. We report the mean and standard deviation over 5 random seeds.

| VisA (AS)  | $K = 0$  |                 | $K = 1$  |                 | $K = 2$  |                 | $K = 4$  |                 |
|------------|----------|-----------------|----------|-----------------|----------|-----------------|----------|-----------------|
|            | WinCLIP  | FADE            | WinCLIP+ | FADE            | WinCLIP+ | FADE            | WinCLIP+ | FADE            |
| Candle     | 83.5±0.0 | 93.5±0.0        | 94.0±0.4 | 97.0±0.2        | 94.2±0.2 | 97.1±0.2        | 94.4±0.2 | 97.2±0.1        |
| Capsules   | 35.3±0.0 | 42.7±0.0        | 73.6±3.5 | 80.8±1.1        | 75.9±1.9 | 82.1±0.8        | 77.0±1.4 | 82.3±0.7        |
| Cashew     | 76.4±0.0 | 89.3±0.0        | 91.1±0.8 | 90.1±1.5        | 90.4±0.6 | 89.5±1.3        | 91.3±0.9 | 86.7±2.8        |
| Chewinggum | 70.4±0.0 | 91.9±0.0        | 91.0±0.5 | 87.0±0.5        | 90.9±0.7 | 86.8±0.3        | 91.0±0.4 | 86.4±0.5        |
| Fryum      | 77.4±0.0 | 90.7±0.0        | 89.1±1.0 | 92.5±0.5        | 89.3±0.2 | 92.6±0.6        | 89.7±0.5 | 92.6±0.2        |
| Macaroni1  | 34.3±0.0 | 91.6±0.0        | 84.6±2.3 | 92.7±2.6        | 85.2±1.4 | 94.4±0.8        | 86.8±0.8 | 94.6±0.4        |
| Macaroni2  | 21.4±0.0 | 84.5±0.0        | 89.3±2.4 | 82.0±5.2        | 88.6±1.7 | 83.1±2.1        | 90.5±1.3 | 85.8±2.4        |
| PCB1       | 26.3±0.0 | 70.2±0.0        | 82.5±6.0 | 90.5±0.7        | 83.8±5.0 | 90.2±1.9        | 87.9±2.1 | 88.9±2.1        |
| PCB2       | 37.2±0.0 | 61.8±0.0        | 73.6±1.5 | 86.1±1.5        | 76.2±0.9 | 87.9±0.5        | 78.0±1.3 | 89.6±0.4        |
| PCB3       | 56.1±0.0 | 72.9±0.0        | 79.5±2.5 | 87.0±1.7        | 82.3±1.8 | 88.9±1.2        | 84.2±1.0 | 89.7±0.6        |
| PCB4       | 80.4±0.0 | 67.7±0.0        | 76.6±4.1 | 85.3±5.7        | 81.7±1.2 | 88.4±3.2        | 84.2±0.7 | 90.1±1.3        |
| Pipe fryum | 82.3±0.0 | 94.6±0.0        | 96.1±0.6 | 95.9±0.9        | 96.2±0.6 | 96.1±0.5        | 96.6±0.2 | 96.3±0.4        |
| Mean       | 56.8±0.0 | <b>79.3±0.0</b> | 85.1±2.1 | <b>88.9±0.7</b> | 86.2±1.4 | <b>89.8±0.4</b> | 87.6±0.9 | <b>90.0±0.4</b> |

Table 12: Comparison of anomaly segmentation (AS) performance in terms of class-wise PRO on VisA. We report the mean and standard deviation over 5 random seeds.

| VisA (AS)  | $K = 0$  |                 | $K = 1$  |                 | $K = 2$   |                 | $K = 4$         |          |
|------------|----------|-----------------|----------|-----------------|-----------|-----------------|-----------------|----------|
|            | WinCLIP  | FADE            | WinCLIP+ | FADE            | WinCLIP+  | FADE            | WinCLIP+        | FADE     |
| $F_1$ -max |          |                 |          |                 |           |                 |                 |          |
| Candle     | 22.5±0.0 | 13.6±0.0        | 42.7±1.7 | 30.1±1.2        | 42.2±0.8  | 30.0±1.3        | 43.0±0.9        | 30.2±1.0 |
| Capsules   | 9.2±0.0  | 11.8±0.0        | 58.2±1.3 | 31.4±0.9        | 57.0±3.7  | 35.0±2.3        | 59.8±1.8        | 37.9±2.3 |
| Cashew     | 13.2±0.0 | 13.0±0.0        | 59.5±2.1 | 69.0±2.4        | 60.5±2.4  | 71.3±1.6        | 62.3±1.1        | 72.9±1.3 |
| Chewinggum | 41.1±0.0 | 45.9±0.0        | 65.3±0.5 | 65.9±1.7        | 64.8±0.9  | 65.1±1.4        | 65.2±0.2        | 63.2±1.0 |
| Fryum      | 22.1±0.0 | 32.2±0.0        | 50.8±1.8 | 49.7±0.4        | 54.8±1.7  | 50.4±1.0        | 56.5±0.6        | 52.0±0.5 |
| Macaroni1  | 7.0±0.0  | 17.9±0.0        | 34.1±1.7 | 27.2±1.5        | 33.2±1.9  | 28.9±1.4        | 33.8±0.9        | 29.3±1.5 |
| Macaroni2  | 1.0±0.0  | 15.3±0.0        | 34.4±3.0 | 6.9±3.0         | 29.9±3.4  | 7.0±1.8         | 35.1±2.5        | 11.7±2.4 |
| PCB1       | 2.4±0.0  | 6.4±0.0         | 25.9±2.6 | 59.8±3.6        | 34.6±16.2 | 63.9±6.4        | 50.9±20.4       | 70.8±6.8 |
| PCB2       | 4.7±0.0  | 2.8±0.0         | 18.7±1.5 | 38.5±1.4        | 24.0±1.1  | 41.6±1.2        | 27.8±1.9        | 43.7±0.7 |
| PCB3       | 10.3±0.0 | 3.3±0.0         | 31.2±6.7 | 36.7±2.1        | 37.1±2.8  | 41.9±1.9        | 42.5±1.1        | 45.3±0.8 |
| PCB4       | 32.0±0.0 | 7.6±0.0         | 22.8±2.9 | 30.9±4.0        | 36.6±2.4  | 35.6±1.4        | 31.9±3.0        | 36.6±1.3 |
| Pipe fryum | 12.3±0.0 | 30.2±0.0        | 51.8±2.0 | 61.5±3.8        | 53.6±2.6  | 62.1±3.3        | 55.1±1.1        | 62.7±1.4 |
| Mean       | 14.8±0.0 | <b>16.7±0.0</b> | 41.3±2.3 | <b>42.3±0.5</b> | 43.5±3.3  | <b>44.4±0.9</b> | <b>47.0±3.0</b> | 46.4±0.7 |

Table 13: Comparison of anomaly segmentation (AS) performance in terms of class-wise  $F_1$ -max on VisA. We report the mean and standard deviation over 5 random seeds.

## 4 Comparison with other state-of-the-art methods

Tab. 14 and 15 show additional quantitative AC and AS results comparing FADE with other state-of-the-art methods such as AnomalyCLIP [10], AnomalyGPT [10] and APRIL-GAN [10]. FADE performs competitively even though these other methods require training using additional anomaly detection datasets while FADE does not need any further training.

## 5 Ablation study on CLIP vs GEM embeddings

Tab. 16 and 17 compare the results of using CLIP or GEM embeddings for FADE under different settings and scenarios. The result motivates the choice of CLIP or GEM embeddings used in Fig. 2a-d of the main paper. GEM embeddings give better results for language-guided AS and vision-guided 0-shot AS. CLIP embeddings give better results for language-guided AC and vision-guided few-shot AC and AS.

| Anomaly Classification |             | MVTec-AD        |                 |                 | VisA            |                 |                 |
|------------------------|-------------|-----------------|-----------------|-----------------|-----------------|-----------------|-----------------|
| Setup                  | Method      | AUROC           | AUPR            | F1-max          | AUROC           | AUPR            | F1-max          |
| 0-shot                 | WinCLIP     | <b>91.8±0.0</b> | <b>96.5±0.0</b> | <b>92.9±0.0</b> | <u>78.1±0.0</u> | 81.2±0.0        | <b>79.0±0.0</b> |
|                        | AnomalyClip | <u>91.5±0.0</u> | <u>96.2±0.0</u> | –               | <b>82.1±0.0</b> | <b>85.4±0.0</b> | –               |
|                        | APRIL-GAN   | 86.1±0.0        | 93.5±0.0        | 90.4±0.0        | 78.0±0.0        | <u>81.4±0.0</u> | <u>78.7±0.0</u> |
|                        | FADE (ours) | 90.0±0.0        | 95.6±0.0        | <u>92.4±0.0</u> | 75.6±0.0        | 78.5±0.0        | 78.6±0.0        |
| 1-shot                 | PatchCore   | 83.4±3.0        | 92.2±1.5        | 90.5±1.5        | 79.9±2.9        | 82.8±2.3        | 81.7±1.6        |
|                        | WinCLIP+    | 93.1±2.0        | <u>96.5±0.9</u> | <u>93.7±1.1</u> | 83.8±4.0        | 85.1±4.0        | 83.1±1.7        |
|                        | AnomalyGPT  | <b>94.1±1.1</b> | –               | –               | 87.4±0.8        | –               | –               |
|                        | APRIL-GAN   | 92.0±0.3        | 95.8±0.2        | 92.4±0.2        | <b>91.2±0.8</b> | <b>93.3±0.8</b> | <b>86.9±0.6</b> |
|                        | FADE (ours) | <u>93.9±0.7</u> | <b>96.8±0.3</b> | <b>94.8±0.2</b> | 86.7±2.0        | <u>87.9±1.5</u> | <u>84.7±0.8</u> |
| 2-shot                 | PatchCore   | 86.3±3.3        | 93.8±1.7        | 92.0±1.5        | 81.6±4.0        | 84.8±3.2        | 82.5±1.8        |
|                        | WinCLIP+    | 94.4±1.3        | <u>97.0±0.7</u> | <u>94.4±0.8</u> | 84.6±2.4        | 85.8±2.7        | 83.0±1.4        |
|                        | AnomalyGPT  | <b>95.5±0.8</b> | –               | –               | 88.6±0.7        | –               | –               |
|                        | APRIL-GAN   | 92.4±0.3        | 96.0±0.2        | 92.6±0.1        | <b>92.2±0.3</b> | <b>94.2±0.3</b> | <b>87.7±0.3</b> |
|                        | FADE (ours) | <u>95.2±1.0</u> | <b>97.6±0.5</b> | <b>95.0±0.4</b> | <u>89.2±0.4</u> | <u>90.2±0.2</u> | <u>85.9±0.6</u> |
| 4-shot                 | PatchCore   | 88.8±2.6        | 94.5±1.5        | 92.6±1.6        | 85.3±2.1        | 87.5±2.1        | 84.3±1.3        |
|                        | WinCLIP+    | <u>95.2±1.3</u> | <u>97.3±0.6</u> | <u>94.7±0.8</u> | 87.3±1.8        | 88.8±1.8        | 84.2±1.6        |
|                        | AnomalyGPT  | <b>96.3±0.3</b> | –               | –               | 90.6±0.7        | –               | –               |
|                        | APRIL-GAN   | 92.8±0.2        | 96.3±0.1        | 92.8±0.1        | <b>92.6±0.4</b> | <b>94.5±0.3</b> | <b>88.4±0.5</b> |
|                        | FADE (ours) | <b>96.3±0.4</b> | <b>98.1±0.2</b> | <b>95.5±0.4</b> | <u>90.7±0.3</u> | <u>91.9±0.4</u> | <u>87.0±0.2</u> |

Table 14: Additional comparison of AC performance on MVTec-AD and VisA. We report the mean and standard deviation over 5 random seeds. Bold and underline denote the best and second best results respectively. AnomalyCLIP [10], AnomalyGPT [10] and APRIL-GAN [10] use additional datasets for training. WinCLIP [10] and FADE require no training.

| Anomaly Segmentation |             | MVTec-AD        |                 |                 | VisA            |                 |                 |
|----------------------|-------------|-----------------|-----------------|-----------------|-----------------|-----------------|-----------------|
| Setup                | Method      | pAUROC          | PRO             | F1-max          | pAUROC          | PRO             | F1-max          |
| 0-shot               | WinCLIP     | 85.1±0.0        | 64.6±0.0        | 31.7±0.0        | 79.6±0.0        | 56.8±0.0        | 14.8±0.0        |
|                      | AnomalyCLIP | <b>91.1±0.0</b> | 81.4±0.0        | –               | <b>95.5±0.0</b> | <b>87.0±0.0</b> | –               |
|                      | APRIL-GAN   | 87.6±0.0        | 44.0±0.0        | <b>43.3±0.0</b> | 94.2±0.0        | 86.8±0.0        | <b>32.3±0.0</b> |
|                      | FADE (ours) | 89.6±0.0        | <b>84.5±0.0</b> | 39.8±0.0        | 91.5±0.0        | 79.3±0.0        | 16.7±0.0        |
| 1-shot               | PatchCore   | 92.0±1.0        | 79.7±2.0        | 50.4±2.1        | 95.4±0.6        | 80.5±2.5        | 38.0±1.9        |
|                      | WinCLIP+    | 95.2±0.5        | 87.1±1.2        | <b>55.9±2.7</b> | 96.4±0.4        | 85.1±2.1        | 41.3±2.3        |
|                      | AnomalyGPT  | 95.3±0.1        | –               | –               | 96.2±0.1        | –               | –               |
|                      | APRIL-GAN   | 95.1±0.1        | <b>90.6±0.2</b> | 54.2±0.0        | 96.0±0.0        | <b>90.0±0.1</b> | 38.5±0.3        |
|                      | FADE (ours) | <b>95.4±0.3</b> | 88.3±0.3        | 54.6±1.1        | <b>97.5±0.1</b> | 88.9±0.7        | <b>42.3±0.5</b> |
| 2-shot               | PatchCore   | 93.3±0.6        | 82.3±1.3        | 53.0±1.7        | 96.1±0.5        | 82.6±2.3        | 41.0±3.9        |
|                      | WinCLIP+    | <b>96.0±0.3</b> | 88.4±0.9        | <b>58.4±1.7</b> | 96.8±0.3        | 86.2±1.4        | 43.5±3.3        |
|                      | AnomalyGPT  | 95.6±0.2        | –               | –               | 96.4±0.1        | –               | –               |
|                      | APRIL-GAN   | 95.5±0.0        | <b>91.3±0.1</b> | 55.9±0.5        | 96.2±0.0        | <b>90.1±0.1</b> | 39.3±0.2        |
|                      | FADE (ours) | 95.8±0.2        | 88.9±0.2        | 55.8±1.0        | <b>97.8±0.1</b> | 89.8±0.4        | <b>44.4±0.9</b> |
| 4-shot               | PatchCore   | 94.3±0.5        | 84.3±1.6        | 55.0±1.9        | 96.8±0.3        | 84.9±1.4        | 43.9±3.1        |
|                      | WinCLIP+    | <b>96.2±0.3</b> | 89.0±0.8        | <b>59.5±1.8</b> | 97.2±0.2        | 87.6±0.9        | <b>47.0±3.0</b> |
|                      | AnomalyGPT  | <b>96.2±0.1</b> | –               | –               | 96.7±0.1        | –               | –               |
|                      | APRIL-GAN   | 95.9±0.0        | <b>91.8±0.1</b> | 56.9±0.1        | 96.2±0.0        | <b>90.2±0.1</b> | 40.0±0.1        |
|                      | FADE (ours) | <b>96.2±0.1</b> | 89.5±0.2        | 57.0±0.8        | <b>98.0±0.0</b> | 90.0±0.4        | 46.4±0.7        |

Table 15: Additional comparison of AS performance on MVTec-AD and VisA. We report the mean and standard deviation over 5 random seeds. Bold and underline denote the best and second best results respectively. AnomalyCLIP [14], AnomalyGPT [15] and APRIL-GAN [16] use additional datasets for training. WinCLIP [17] and FADE require no training.

| Anomaly Classification |        |            | AUROC       |             |
|------------------------|--------|------------|-------------|-------------|
| Guidance               | Shot   | Embeddings | MVTec-AD    | VisA        |
| Language               | 0-shot | CLIP       | <b>90.0</b> | <b>75.6</b> |
|                        |        | GEM        | 43.8        | 50.3        |
| Vision                 | 1-shot | CLIP       | <b>90.7</b> | <b>86.0</b> |
|                        |        | GEM        | 87.8        | 79.4        |

Table 16: AC results (AUROC) for using CLIP vs GEM embeddings under different settings.

| Anomaly Segmentation |        |            | pAUROC      |             |
|----------------------|--------|------------|-------------|-------------|
| Guidance             | Shot   | Embeddings | MVTec-AD    | VisA        |
| Language             | 0-shot | CLIP       | 18.0        | 13.9        |
|                      |        | GEM        | <b>86.5</b> | <b>87.0</b> |
| Vision               | 0-shot | CLIP       | 74.6        | 81.6        |
|                      |        | GEM        | <b>86.6</b> | <b>87.1</b> |
| Vision               | 1-shot | CLIP       | <b>95.1</b> | <b>97.3</b> |
|                      |        | GEM        | 93.5        | 91.9        |

Table 17: AS results (pAUROC) for using CLIP vs GEM embeddings under different settings.

## 6 Qualitative results

### 6.1 Additional main results

Fig. 7 and 8 show additional qualitative results for 0-shot and 1-shot AS on the MVTec-AD and VisA benchmarks respectively. For most object classes, the AS performance of 1-shot is better than 0-shot since the additional normal reference image provides important visual cues that better capture the concept of normality. This is especially important for object classes (E.g. cable, metal nut, transistor, pcb) that sometimes contain logical anomalies which cannot be detected in a 0-shot setting. In addition, object classes like pill contains deviations (E.g. spots on the pill) that can only be defined as normal when a reference image is available.

Interestingly, for a few other object classes such as grid and wood, we observe the opposite where 0-shot performance is better than 1-shot. This is because these two object classes contain textural patterns that are orientation-specific. Under the 1-shot setting, a normal reference image of wood may contain wood fibres that are oriented in a direction different from a normal query image. As such, the vision-guided AS based on the memory bank built from the visual patches of the reference image is not ideal since we do not want to pick up the differences in fibre orientation as an anomaly. In contrast, under the 0-shot setting, the memory bank is built using the patches from the query image itself which all share similar wood fibre orientation. This allows vision-guided AS to be independent of fibre orientation and enables it to focus more on the actual inconsistencies and anomalies within the image, resulting in more accurate and fine-grained segmentation results.

### 6.2 Ablation results

**CLIP vs GEM for zero-shot AS:** Fig. 6 shows the qualitative results of language-guided zero-shot AS on MVTec-AD when CLIP or GEM patch embeddings are used. We observe that CLIP embeddings result in opposite visualisation between the normal and anomalous regions (see “leather” example) and also tend to produce noisier activations. In contrast, GEM embeddings address both issues and generate much better segmentation maps.

**Multi-scale aggregation:** Fig. 9 shows the qualitative AS results on MVTec-AD when different input image scale/size is used. Results are shown for both zero- and one-shot setting. For each setting, both language and vision guidance are used. We observe that a smaller input image size (240) gives a coarser segmentation map, allowing for the detection of larger anomalies. In contrast, a larger input image size (896) produces more fine-grained segmentation map with higher resolution that can identify smaller anomalies. The multi-scale aggregation of all the three segmentation maps with different scales allows for the detection of anomalies with different sizes. It gives the best qualitative results that show fine details on the outline of the anomalous regions and suppress the false positive detection in the background.

**Language vs vision guidance:** Fig. 10 shows the impact of language vs vision guidance on the qualitative results for zero-shot AS. Specifically, vision guidance works better for textural classes (E.g. zipper, wood) that demonstrate repetitive patterns. Anomalies that break such repetition and consistency are detected by visual comparison of patch embeddings within the image. In contrast, language guidance works better for object classes (E.g. screw, toothbrush) where the knowledge and concepts of anomaly learned by the CLIP model are elicited through language. In general, language and vision guidance are complementary and combining them gives the best qualitative results.

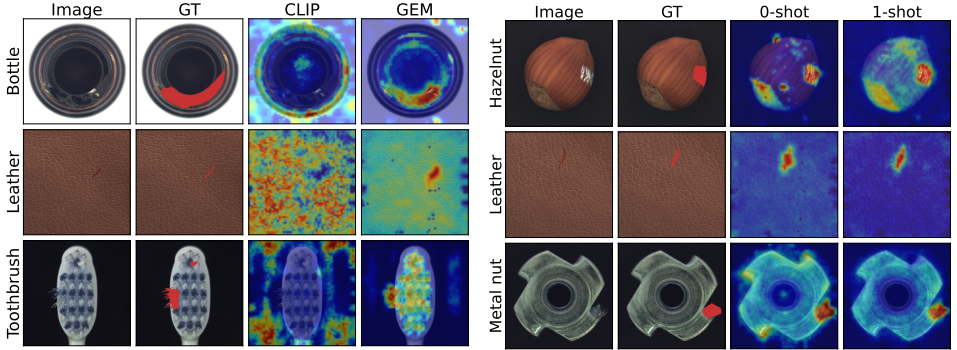

Figure 6: Qualitative results for impact of CLIP vs GEM patch embeddings on language-guided zero-shot AS on MVTec-AD.

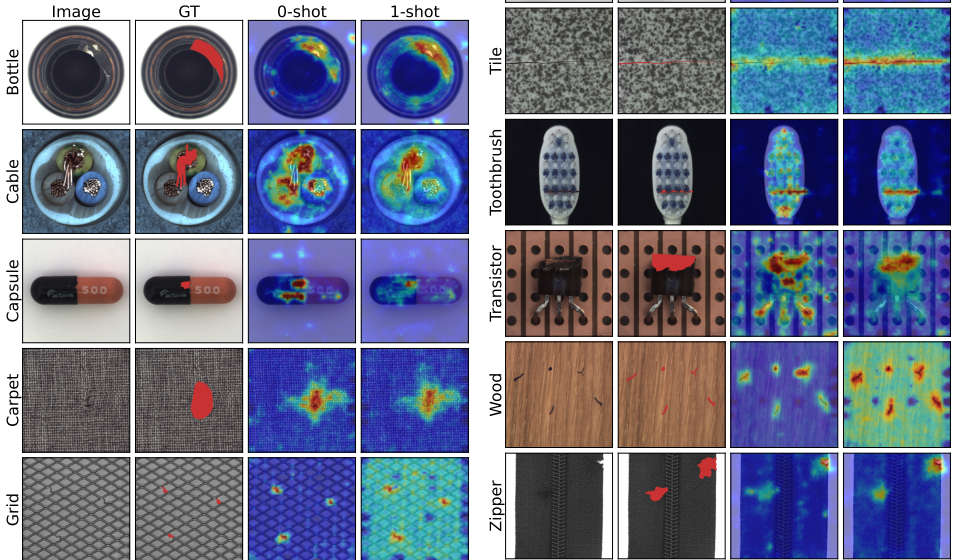

Figure 7: Additional qualitative results for zero-shot and one-shot AS on MVTec-AD.

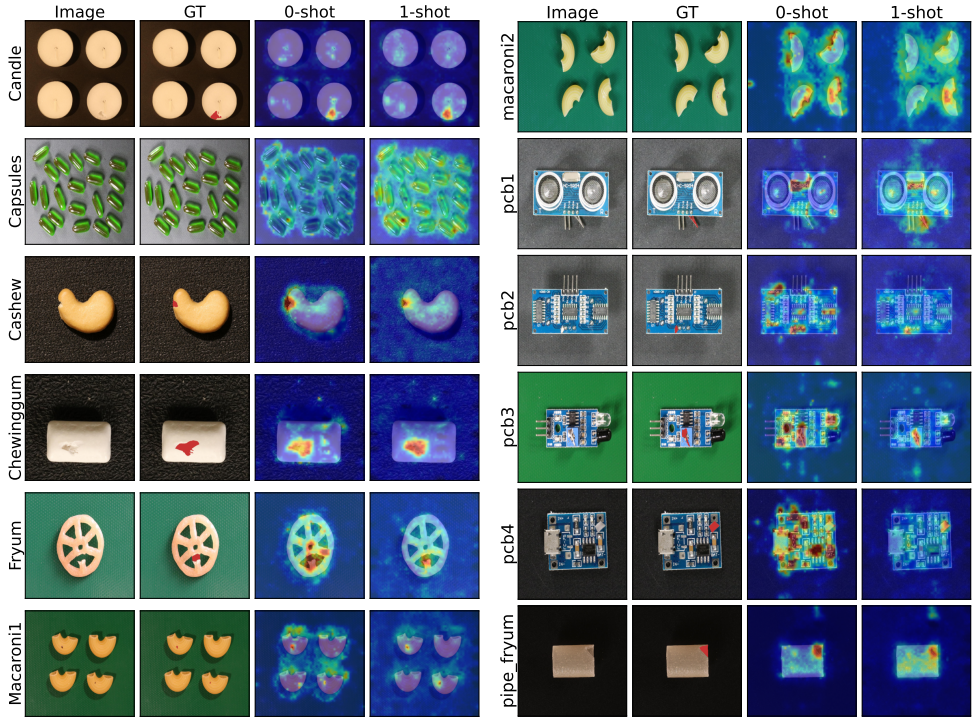

Figure 8: Additional qualitative results for zero-shot and one-shot AS on VisA.

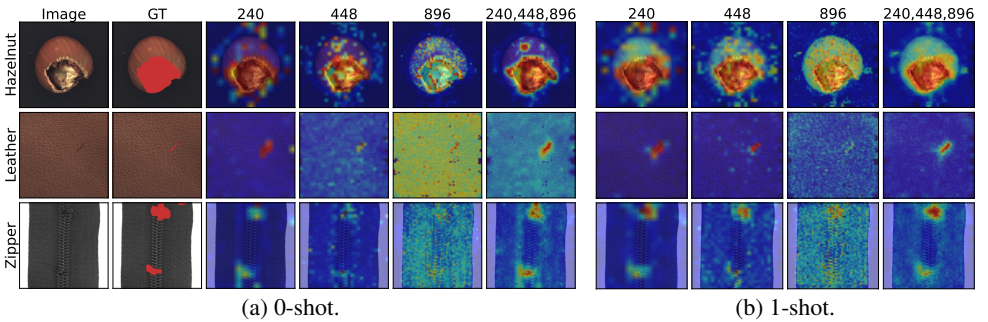

Figure 9: Qualitative AS results for the image scale ablation study on MVTec-AD.

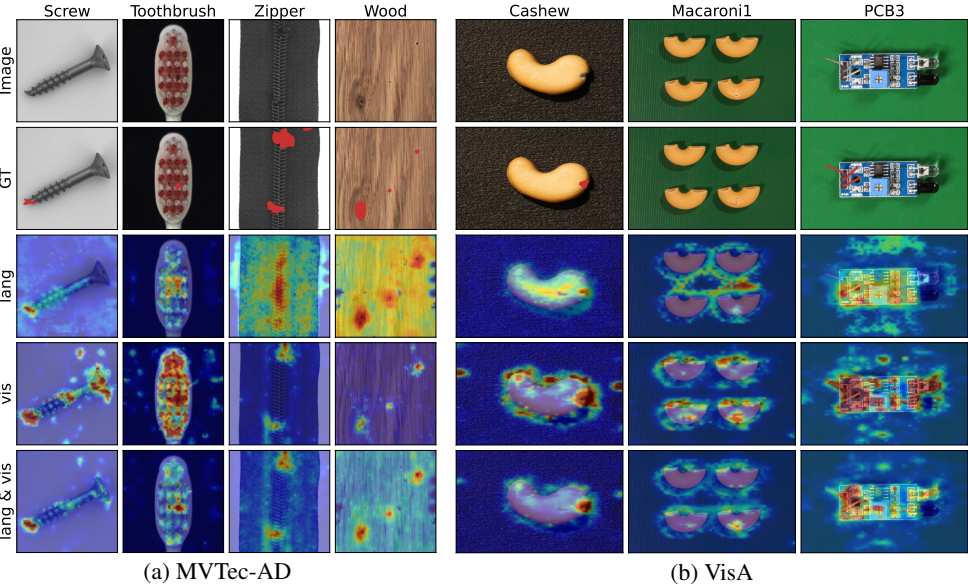

Figure 10: Qualitative results for language- vs vision-guided zero-shot AS.

## References

- [1] Xuhai Chen, Yue Han, and Jiangning Zhang. A zero-/few-shot anomaly classification and segmentation method for CVPR 2023 VAND workshop challenge tracks 1&2: 1st place on zero-shot AD and 4th place on few-shot AD. *arXiv preprint arXiv:2305.17382*, 2023.
- [2] Zhaopeng Gu, Bingke Zhu, Guibo Zhu, Yingying Chen, Ming Tang, and Jinqiao Wang. Anomalygpt: Detecting industrial anomalies using large vision-language models. In *Proceedings of the AAAI Conference on Artificial Intelligence*, volume 38, pages 1932–1940, 2024.
- [3] Jongheon Jeong, Yang Zou, Taewan Kim, Dongqing Zhang, Avinash Ravichandran, and Onkar Dabeer. WinCLIP: Zero-/few-shot anomaly classification and segmentation. In *2023 IEEE/CVF Conference on Computer Vision and Pattern Recognition (CVPR)*, pages 19606–19616, 2023. doi: 10.1109/CVPR52729.2023.01878.
- [4] Qihang Zhou, Guansong Pang, Yu Tian, Shibo He, and Jiming Chen. AnomalyCLIP: Object-agnostic prompt learning for zero-shot anomaly detection. In *The Twelfth International Conference on Learning Representations*, 2024. URL <https://openreview.net/forum?id=buC4E91xZE>.
