# Supplementary material for: FADE: Few-shot/zero-shot Anomaly Detection Engine using Large Vision-Language Model
Source: arXiv:2409.00556 source file (2024-08-31)
Supplement: Supplementary file 3 [file qualitative_additional_main_visa.tex]

\begin{figure}[h]
\centering
\begin{minipage}{0.49\linewidth}
\centering
\includegraphics[width=\textwidth]{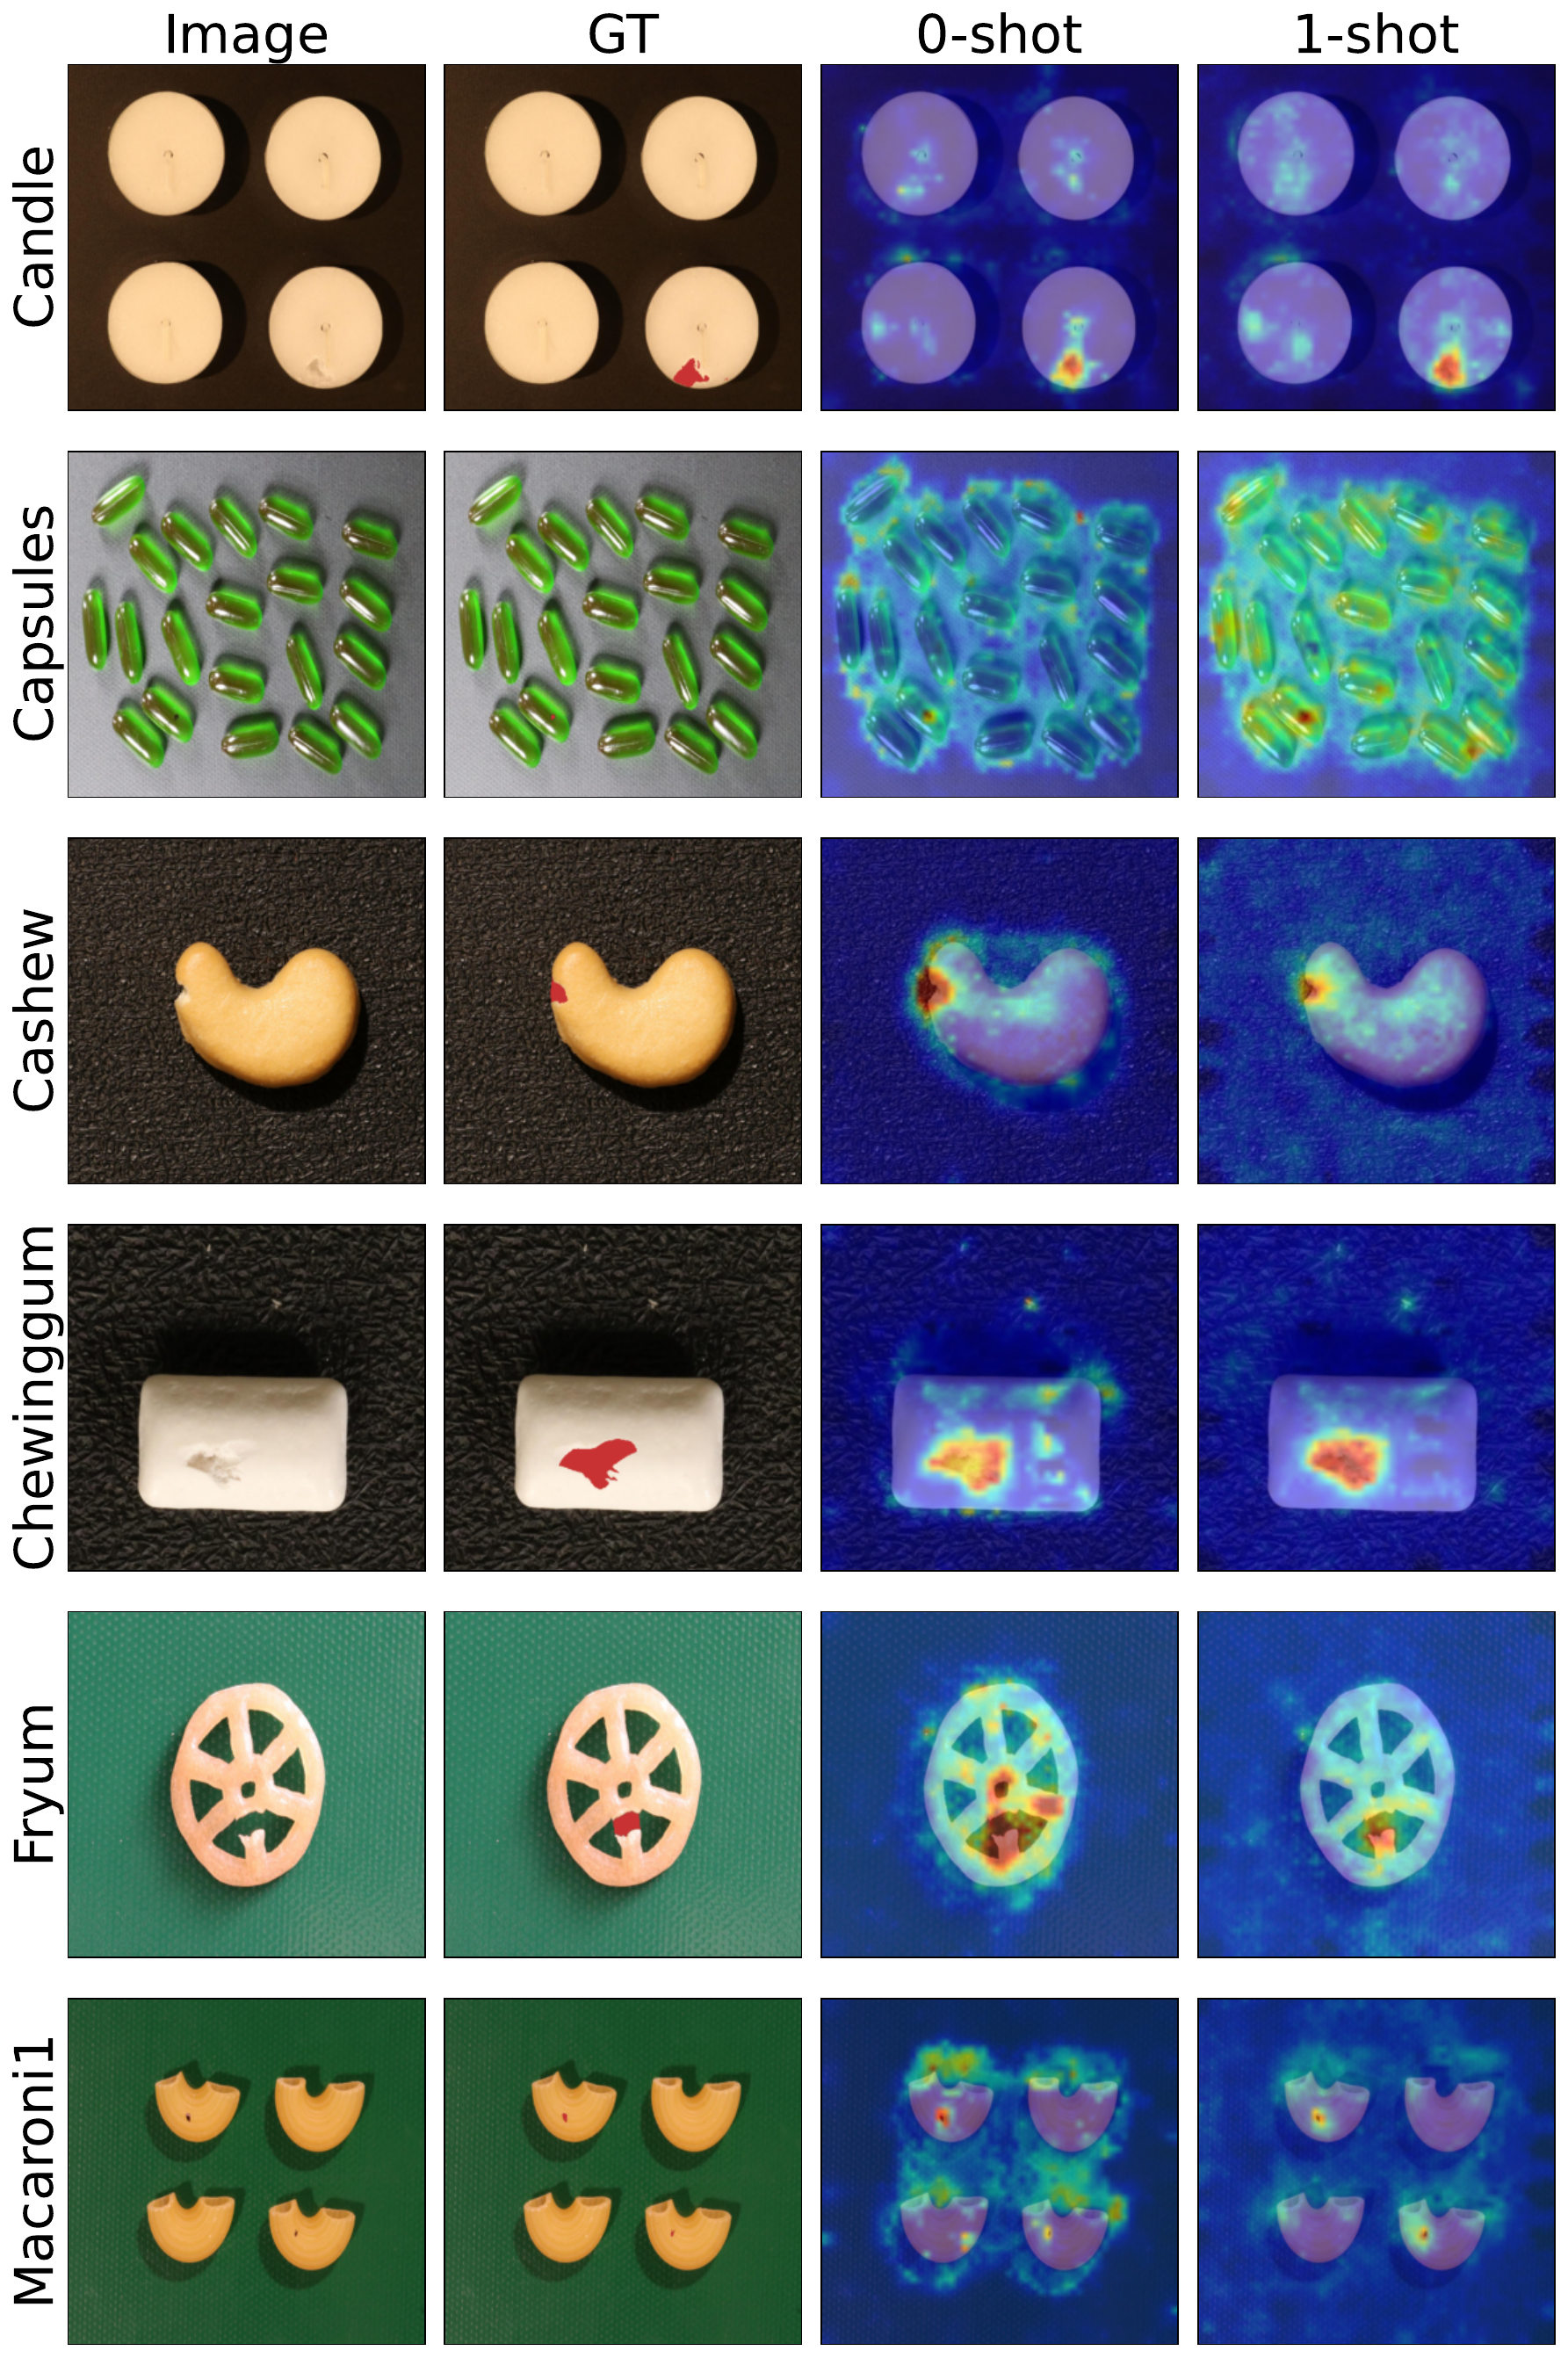}
\captionsetup{labelformat=empty,font=small,skip=1pt}
\caption*{}\label{fig:qual_visa_shots_study_1}
\end{minipage}
\hspace{0.000001\linewidth}
\begin{minipage}{0.49\linewidth}
\centering
\includegraphics[width=\textwidth]{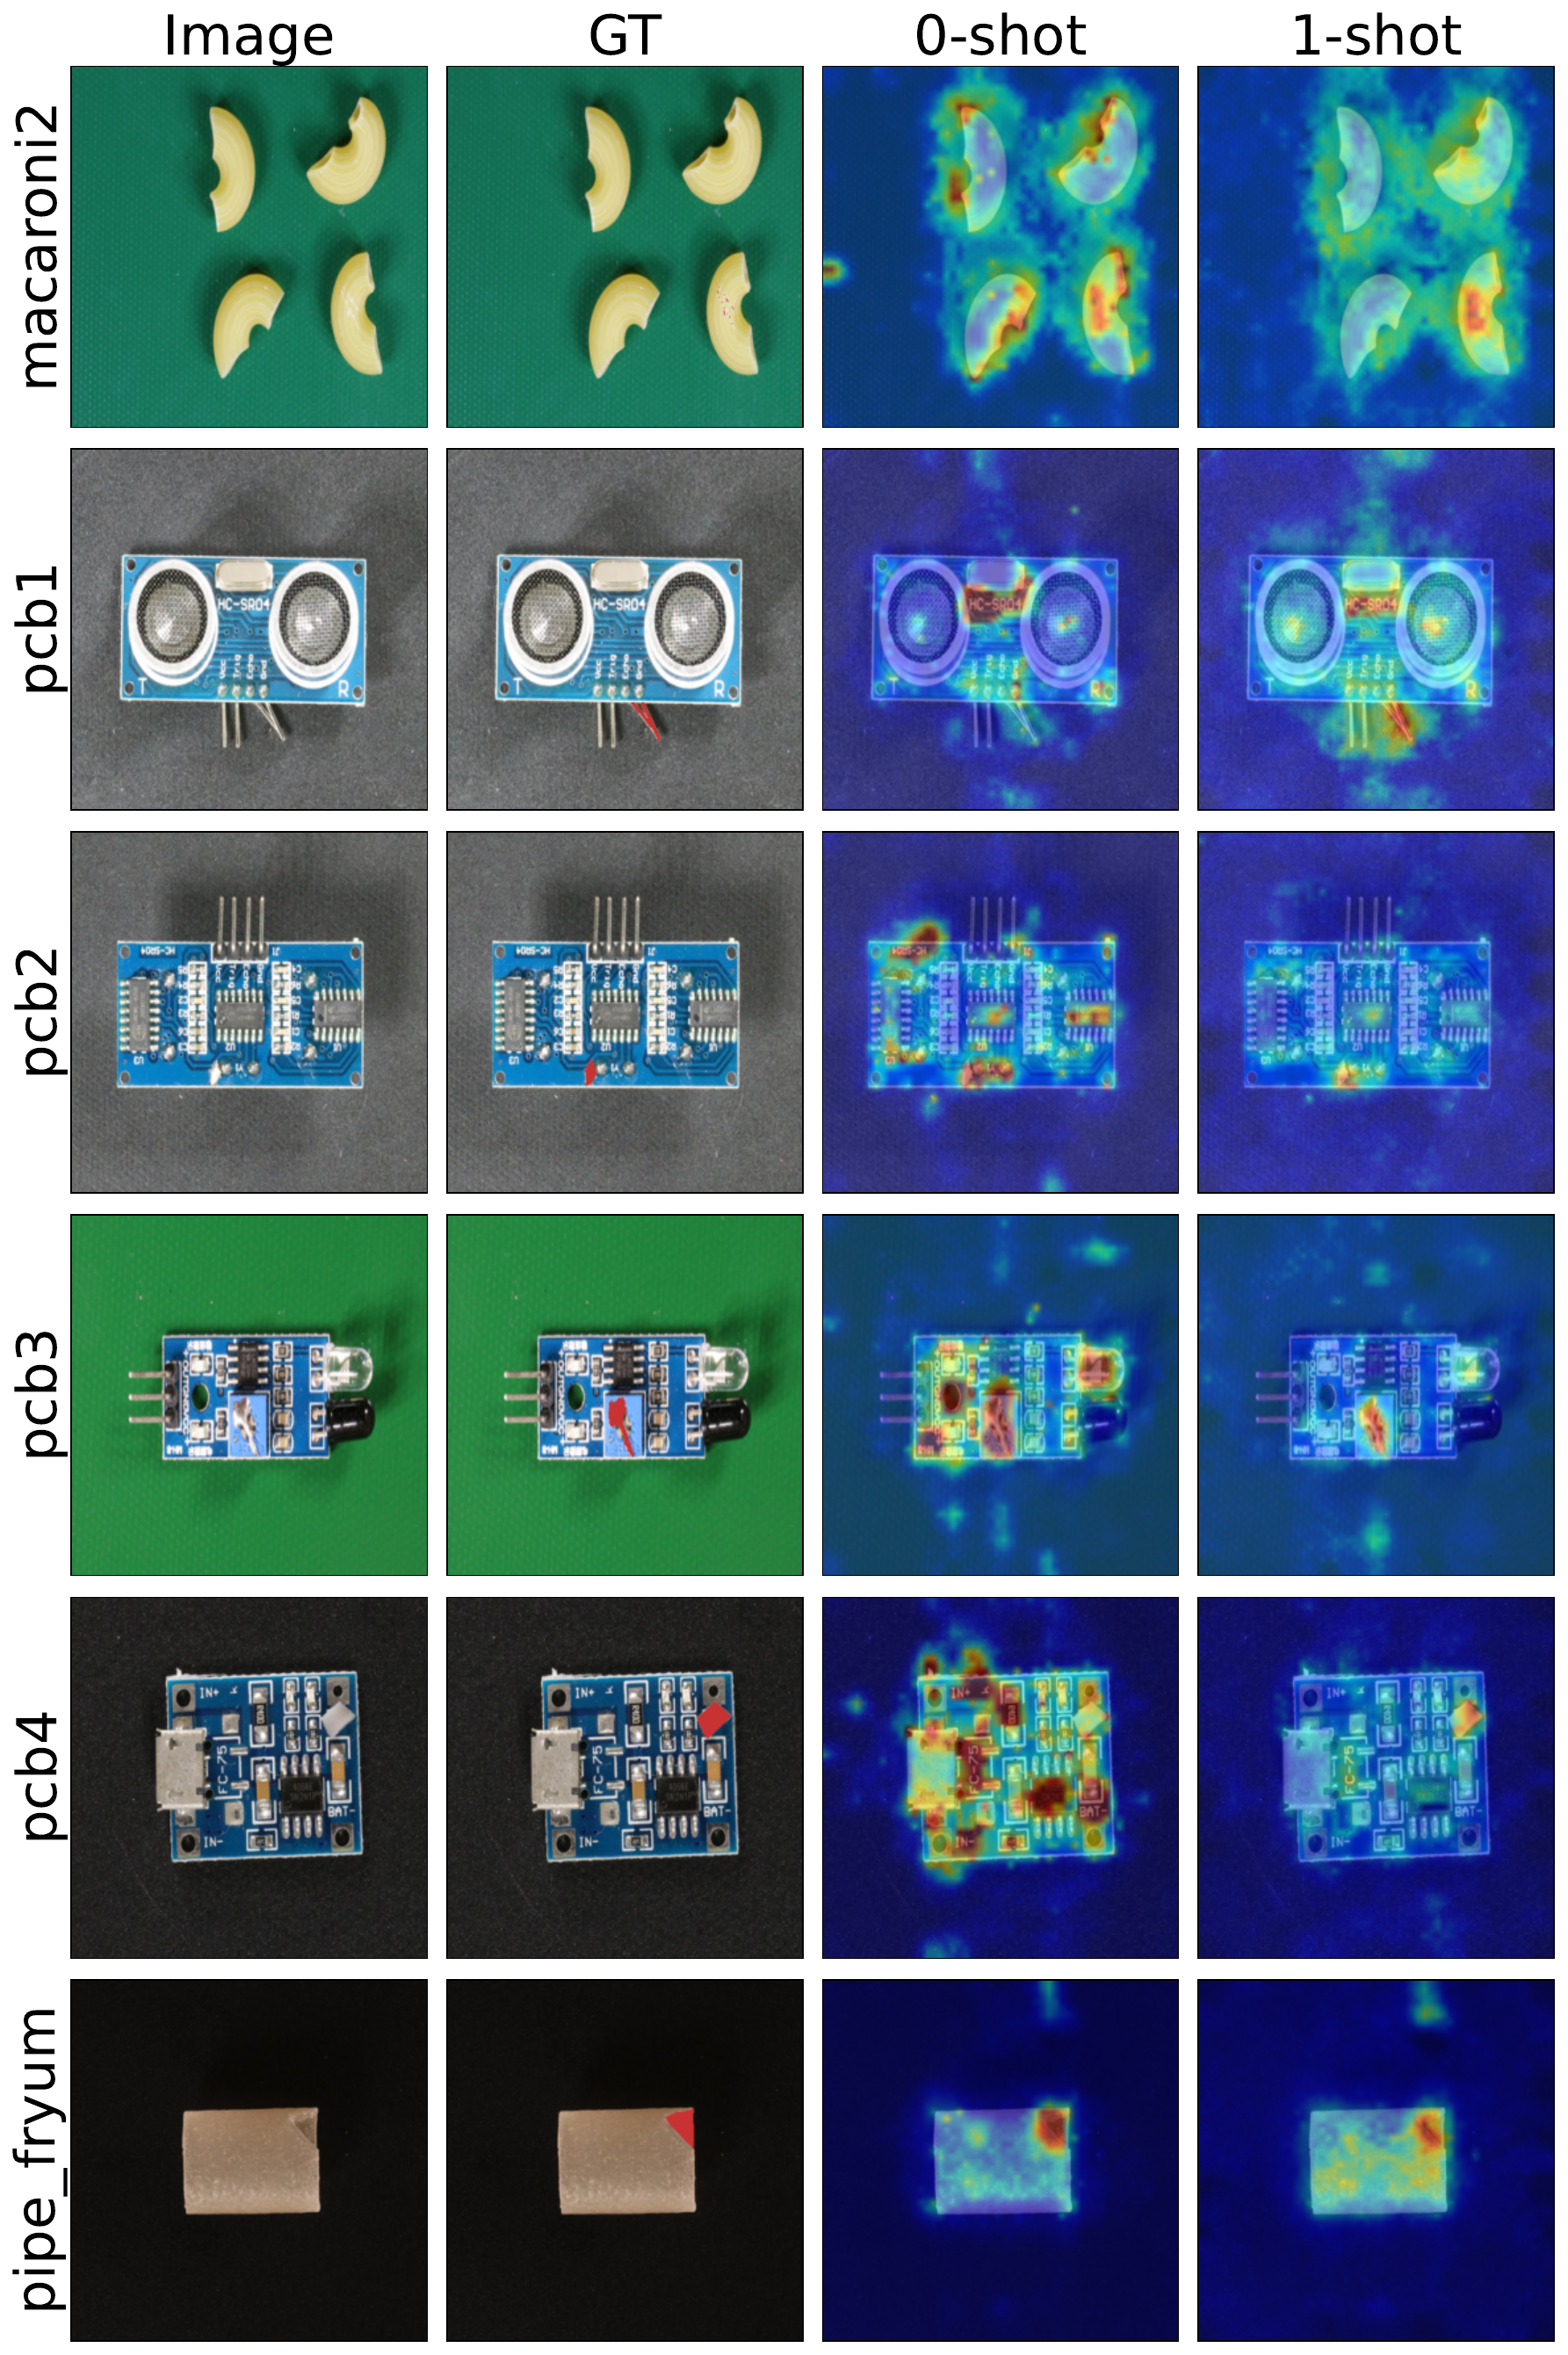}
\captionsetup{labelformat=empty,font=small,skip=1pt}
\caption*{}\label{fig:qual_visa_shots_study_2}
\end{minipage}

\caption{Additional qualitative results for zero-shot and one-shot AS on VisA.}
\label{fig:qualitative_additional_main_visa}
\end{figure}
