# Supplementary material for: FADE: Few-shot/zero-shot Anomaly Detection Engine using Large Vision-Language Model
Source: arXiv:2409.00556 source file (2024-08-31)
Supplement: Supplementary file 4 [file appendix_ac_as_clip_vs_gem.tex]

\begin{table}[h]
    \centering
    \begin{minipage}[c]{0.49\textwidth}
        \centering
        \resizebox{\textwidth}{!}{%
            \begin{tabular}{ccccc}
                \toprule
                \multicolumn{3}{c}{Anomaly Classification} & \multicolumn{2}{c}{AUROC} \\
                \cmidrule(lr){4-5}
                Guidance & Shot & Embeddings & MVTec-AD & VisA \\
                \midrule
                Language & 0-shot & CLIP & \textbf{90.0} & \textbf{75.6}  \\
                & & GEM & 43.8  & 50.3 \\
                \midrule
                Vision & 1-shot & CLIP & \textbf{90.7}  & \textbf{86.0} \\
                & & GEM & 87.8 & 79.4 \\
                \bottomrule
            \end{tabular}
        }
        \caption{
        AC results (AUROC) for using CLIP vs GEM embeddings under different settings.
        }
        \label{tab:appendix_ac_clip_vs_gem}
    \end{minipage}    
    \hfill
    \begin{minipage}[c]{0.49\textwidth}
        \centering
        \resizebox{\textwidth}{!}{%
            \begin{tabular}{ccccc}
                \toprule
                \multicolumn{3}{c}{Anomaly Segmentation} & \multicolumn{2}{c}{pAUROC} \\
                \cmidrule(lr){4-5}
                Guidance & Shot & Embeddings & MVTec-AD & VisA \\
                \midrule
                Language & 0-shot & CLIP & 18.0 & 13.9  \\
                & & GEM & \textbf{86.5}  & \textbf{87.0} \\
                \midrule
                Vision & 0-shot & CLIP & 74.6 & 81.6  \\
                & & GEM & \textbf{86.6}  & \textbf{87.1} \\
                \midrule
                Vision & 1-shot & CLIP & \textbf{95.1}  & \textbf{97.3}  \\
                & & GEM & 93.5 & 91.9 \\
                \bottomrule
            \end{tabular}
        }
        \caption{AS results (pAUROC) for using CLIP vs GEM embeddings under different settings.}
        \label{tab:appendix_as_clip_vs_gem}
    \end{minipage}
\end{table}
