# Supplementary material for: FADE: Few-shot/zero-shot Anomaly Detection Engine using Large Vision-Language Model
Source: arXiv:2409.00556 source file (2024-08-31)
Supplement: Supplementary file 5 [file appendix_ac_clip_vs_gem.tex]

\begin{table}[t]
\begin{center}
\begin{tabular}{lllcc}
\toprule
\multicolumn{3}{c}{Anomaly Classification} & \multicolumn{2}{c}{AUROC} \\
\cmidrule(lr){4-5}
Guidance & Shot & Embeddings & MVTec-AD & VisA \\
\midrule
Language & 0-shot & CLIP & \textbf{90.0} & \textbf{75.6}  \\
& & GEM & 43.8  & 50.3 \\
\midrule
Vision & 1-shot & CLIP & \textbf{90.7}  & \textbf{86.0} \\
& & GEM & 87.8 & 79.4 \\
\bottomrule
\end{tabular}
\end{center}
\caption{
AC results (AUROC) for using CLIP vs GEM embeddings under different settings.
}
\label{tab:appendix_ac_clip_vs_gem}
\end{table}
