# Supplementary material for: FADE: Few-shot/zero-shot Anomaly Detection Engine using Large Vision-Language Model
Source: arXiv:2409.00556 source file (2024-08-31)
Supplement: Supplementary file 6 [file appendix_as_clip_vs_gem.tex]

\begin{table}[t]
\begin{center}
\begin{tabular}{lllcc}
\toprule
\multicolumn{3}{c}{Anomaly Segmentation} & \multicolumn{2}{c}{pAUROC} \\
\cmidrule(lr){4-5}
Guidance & Shot & Embeddings & MVTec-AD & VisA \\
\midrule
Language & 0-shot & CLIP & 18.0 & 13.9  \\
& & GEM & \textbf{86.5}  & \textbf{87.0} \\
\midrule
Vision & 0-shot & CLIP & 74.6 & 81.6  \\
& & GEM & \textbf{86.6}  & \textbf{87.1} \\
\midrule
Vision & 1-shot & CLIP & \textbf{95.1}  & \textbf{97.3}  \\
& & GEM & 93.5 & 91.9 \\
\bottomrule
\end{tabular}
\end{center}
\caption{
AS results (pAUROC) for using CLIP vs GEM embeddings under different settings.
}
\label{tab:appendix_as_clip_vs_gem}
\end{table}
