# Supplementary material for: FADE: Few-shot/zero-shot Anomaly Detection Engine using Large Vision-Language Model
Source: arXiv:2409.00556 source file (2024-08-31)
Supplement: Supplementary file 7 [file lang_vis_aggregation_supplementary.tex]

\begin{table}[h]
    \centering
    \resizebox{0.64\textwidth}{!}{%
        \begin{tabular}{ccccc}
        \toprule
        Task & Shot & Aggregation & $\alpha$ & $\beta$  \\
        \midrule
        AC & 0-shot & $s^{lang}$ & - & -  \\
        \cmidrule(lr){2-5}
        & k-shot & $(1-\alpha)s^{lang}+(1-\alpha) \beta s^{vis,k}$ & 0.5 & 3.5  \\
        \midrule
        AS & 0-shot & $(1-\alpha)\boldsymbol{M}^{lang}+(1-\alpha) \beta \boldsymbol{M}^{vis,0}$ & 0.5 & 80  \\
        \cmidrule(lr){2-5}
        & k-shot & $(1-\alpha)\boldsymbol{M}^{lang}+(1-\alpha) \beta \boldsymbol{M}^{vis,k}$ & 0.85 & 3.5  \\
        \bottomrule
        \end{tabular}
    }
    \caption{Aggregation of language and vision guidance under different settings.}
    \label{tab:lang_vis_aggregation_supp}
\end{table}
